# Supplementary material for: Simultaneous Detection of Signal Regions Using Quadratic Scan Statistics With Applications in Whole Genome Association Studies
Source: arXiv:1710.05021 source file (2019-07-25)
Supplement: Supplementary file 1 [file supplementary_material_v2.pdf]

# Supplementary Material

## Contents

|          |                                                  |           |
|----------|--------------------------------------------------|-----------|
| <b>1</b> | <b>Supplementary Note</b>                        | <b>2</b>  |
| 1.1      | Bound of Empirical Threshold . . . . .           | 3         |
| 1.2      | Consistency of Signal Region Detection . . . . . | 7         |
| <b>2</b> | <b>Supplementary Figures</b>                     | <b>15</b> |
| <b>3</b> | <b>Supplementary Tables</b>                      | <b>21</b> |

# 1 Supplementary Note

In this supplementary note, we give the detail proof of the theorems in the paper. In order to proof the theorem, we introduce the following three lemmas first.

**Lemma 1 (Refinement of Bernstein's Inequality (Petrov 1968))** *Consider a sequence of independent random variables  $\{\mathbf{X}_j\}, j = 1, 2, \dots$ . Assume  $\mathbb{E}(\mathbf{X}_j) = 0$ ,  $\mathbb{E}(\mathbf{X}_j^2) = \sigma_j^2$  and  $L_j(z) = \log(\mathbb{E}(\exp(z\mathbf{X}_j)))$ . We introduce the following notation:*

$$\mathbf{S}_n = \sum_{j=1}^n \mathbf{X}_j, \quad B_n = \sum_{j=1}^n \sigma_j^2, \quad F_n(x) = \mathbb{P}(\mathbf{S}_n < x\sqrt{B_n}), \quad \Phi(x) = \frac{1}{\sqrt{2\pi}} \int_{-\infty}^x \exp(-\frac{t^2}{2}) dt.$$

If the following three conditions hold:

- (1) There exists positive constants  $A, c_1, c_2, \dots$  such that  $|L_j(z)| \leq c_j$  for  $|z| < A, j = 1, 2, \dots$ ,
- (2)  $\limsup_{n \rightarrow \infty} \frac{1}{n} \sum_{j=1}^n c_j^{\frac{3}{2}} < \infty$ ,
- (3)  $\liminf_{n \rightarrow \infty} \frac{B_n}{n} > 0$ ,

then there exists a positive constant  $w$  such that for sufficiently large  $n$ ,

$$1 - F_n(x) = [1 - \Phi(x)] \exp \left\{ \frac{x^3}{\sqrt{n}} \lambda_n \left( \frac{x}{\sqrt{n}} \right) \right\} (1 + l_1 w)$$

$$F_n(-x) = \Phi(-x) \exp \left\{ -\frac{x^3}{\sqrt{n}} \lambda_n \left( -\frac{x}{\sqrt{n}} \right) (1 + l_2 w) \right\}$$

in the region  $0 \leq x \leq w\sqrt{n}$ . Here  $|l_1| \leq l$  and  $|l_2| \leq l$  being some constant.

The next two lemmas are two inequalities for the tail probability of normal distribution and chi-square distribution, respectively.

**Lemma 2 (Mills' Ratio Inequality)** *For arbitrary positive number  $x > 0$ , the inequalities*

$$\frac{x}{1+x^2} \exp(-\frac{x^2}{2}) < \int_x^\infty \exp(-\frac{u^2}{2}) du < \frac{1}{x} \exp(-\frac{x^2}{2}).$$

**Lemma 3 (Exponential inequality for chi-square distribution(Laurent and Massart 2000))**

*Let  $\mathbf{Y}_1, \dots, \mathbf{Y}_D$  be i.i.d. standard Gaussian variables. Let  $a_1, \dots, a_D$  be nonnegative constant. We set*

$$\|\mathbf{a}\|_\infty = \sup_{1 \leq i \leq D} |a_i| \quad \|\mathbf{a}\|_2^2 = \sum_{i=1}^D a_i^2.$$

*Let  $\mathbf{Z} = \sum_{i=1}^D a_i(\mathbf{Y}_i^2 - 1)$ , then the following inequalities hold for any positive  $x$ :*

$$\mathbb{P}(\mathbf{Z} \geq 2\|\mathbf{a}\|_2\sqrt{x} + 2\|\mathbf{a}\|_\infty x) \leq \exp(-x),$$

$$\mathbb{P}(\mathbf{Z} \leq -2\|\mathbf{a}\|_2\sqrt{x} \leq \exp(-x).$$

## 1.1 Bound of Empirical Threshold

Now we go back to the proof of the main theorem in the paper. First recall the notation of Q-scan procedure. For any vector  $\mathbf{a}$ , set  $\|\mathbf{a}\|_1 = \sum_i |a_i|$ ,  $\|\mathbf{a}\|_2 = \sqrt{\sum_i a_i^2}$  and  $\|\mathbf{a}\|_\infty = \sup_i |a_i|$ . Let  $U_i = \frac{1}{\sqrt{n}} \mathbf{G}_i^T (\mathbf{Y} - \hat{\boldsymbol{\mu}})$  be the score statistic for variant  $i$ ,  $i = 1, 2, \dots, p$ . Under the null hypothesis,  $U_i \sim N(0, \sigma_i^2)$  with  $\sigma_i^2 = \frac{1}{n} \mathbf{G}_i^T \mathbf{P} \mathbf{G}_i$  for all  $i = 1, 2, \dots, p$ , where  $\mathbf{P}$  is the projection matrix in the null model. Assume there exists constant  $c > 0$  such that  $\sigma_i^2 \geq c$ . For any region  $I$ , assume  $\mathbf{U}_I = (U_i)_{i \in I}$  and  $\boldsymbol{\Sigma}_I = \frac{1}{n} \mathbf{G}_I^T \mathbf{P} \mathbf{G}_I$ , then  $\mathbf{U}_I \sim N(0, \boldsymbol{\Sigma}_I)$ . Let  $\boldsymbol{\lambda}_I$  is the eigenvalues of  $\boldsymbol{\Sigma}_I$ , the Q-scan statistic of region is defined as

$$Q(I) = \frac{\sum_{i \in I} U_i^2 - \sum_{i=1}^{|I|} \lambda_{I,i}}{\sqrt{2 \sum_{i=1}^{|I|} \lambda_{I,i}^2}} = \frac{\sum_{i \in I} U_i^2 - \|\boldsymbol{\lambda}_I\|_1}{\sqrt{2} \|\boldsymbol{\lambda}_I\|_2}.$$

We first proof the results of fixed length scan.

**Lemma 4** *If the following conditions (A)-(C) hold,*

(A)  $\max_{|I|=L_p} \|\boldsymbol{\lambda}_I\|_\infty \leq K_0$ , where  $K_0$  is a constant,

(B)  $\frac{L_p}{\log p} \rightarrow \infty$  and  $\frac{\log(L_p)}{\log(p)} \rightarrow 0$ ,

(C)  $\{U_i\}_{i=1}^p$  is  $M_p$ -dependent and  $\frac{\log(M_p)}{\log(p)} \rightarrow 0$ ,

then

$$\frac{\max_{|I|=L_p} Q(I)}{\sqrt{2 \log(p)}} \xrightarrow{p} 1.$$

**Proof** For any  $I$  satisfies that  $|I| = L_p$ , assume  $\boldsymbol{\Omega}_I \boldsymbol{\Sigma}_I \boldsymbol{\Omega}_I^T = \text{diag}(\boldsymbol{\lambda}_I)$  is the SVD of  $\boldsymbol{\Sigma}_I$  where  $\boldsymbol{\Omega}_I$  is an orthogonal matrix. Let  $\tilde{\mathbf{U}}_I = \boldsymbol{\Omega}_I \mathbf{U}_I$ , then  $\tilde{\mathbf{U}}_I \sim N(0, \text{diag}(\boldsymbol{\lambda}_I))$  and  $\tilde{\mathbf{U}}_I^T \tilde{\mathbf{U}}_I = \mathbf{U}_I^T \mathbf{U}_I$ . Hence, for  $\epsilon > 0$ ,

$$\begin{aligned} \mathbb{P}(Q(I) > (1 + \epsilon) \sqrt{2 \log(p)}) &= \mathbb{P}\left(\sum_{i \in I} U_i^2 - \|\boldsymbol{\lambda}_I\|_1 > 2(2 + \epsilon) \|\boldsymbol{\lambda}_I\|_2 \sqrt{\log(p)}\right) \\ &= \mathbb{P}\left(\sum_{i \in I} \lambda_{I,i} \left(\frac{\tilde{U}_i^2}{\lambda_{I,i}} - 1\right) > 2(1 + \epsilon) \|\boldsymbol{\lambda}_I\|_2 \sqrt{\log(p)}\right). \end{aligned}$$

Note that  $\|\boldsymbol{\lambda}_I\|_2 \geq \|\boldsymbol{\lambda}_I\|_1^2 / \sqrt{|I|} \geq c \sqrt{|I|}$ , by condition (A) and (B), we have

$$(1 + \frac{\epsilon}{2})^2 \|\boldsymbol{\lambda}_I\|_\infty \log(p) = O(\log(p)) = o(\|\boldsymbol{\lambda}_I\|_2 \sqrt{\log(p)}).$$

Then by Lemma 3, for  $p$  sufficiently large,

$$\begin{aligned} &\mathbb{P}\left(\sum_{i \in I} \lambda_{I,i} \left(\frac{\tilde{U}_i^2}{\lambda_{I,i}} - 1\right) > 2(1 + \epsilon) \|\boldsymbol{\lambda}_I\|_2 \sqrt{\log(p)}\right) \\ &\leq \mathbb{P}\left(\sum_{i \in I} \lambda_{I,i} \left(\frac{\tilde{U}_i^2}{\lambda_{I,i}} - 1\right) > 2(1 + \frac{\epsilon}{2})^2 \|\boldsymbol{\lambda}_I\|_2 \sqrt{\log(p)} + 2(1 + \frac{\epsilon}{2}) \|\boldsymbol{\lambda}_I\|_\infty \log(p)\right) \\ &\leq \exp\{-(1 + \frac{\epsilon}{2})^2 \log(p)\}. \end{aligned}$$

Hence, using Boole's inequality,

$$\mathbb{P}\left(\max_{|I|=L_p} Q(I) > (1+\epsilon)\sqrt{2\log(p)}\right) \leq \sum_{|I|=L_p} \mathbb{P}\left(Q(I) > (1+\epsilon)\sqrt{2\log(p)}\right) \leq p \times \exp\left\{-\left(1+\frac{\epsilon}{2}\right)^2 \log(p)\right\} = o(1) \quad (1)$$

On the other hand,

$$\begin{aligned} \mathbb{P}\left(\max_{|I|=L_p} Q(I) < (1-\epsilon)\sqrt{2\log(p)}\right) &= \mathbb{P}\left(\bigcap_{|I|=L_p} \{Q(I) < (1-\epsilon)\sqrt{2\log(p)}\}\right) \\ &= 1 - \mathbb{P}\left(\bigcup_{|I|=L_p} \{Q(I) \geq (1-\epsilon)\sqrt{2\log(p)}\}\right) \end{aligned}$$

Let  $I_k = \{k, k+1, \dots, k+L_p-1\}$  and  $A_k = \left\{\frac{\sum_{i \in I_k} U_i^2 - \|\lambda_{I_k}\|_1}{\sqrt{2}\|\lambda_{I_k}\|_2} \geq (1-\epsilon)\sqrt{2\log(p)}\right\}$ , by Chung-Erdős inequality,

$$\mathbb{P}\left(\bigcup_{|I|=L_p} \{Q(I) \geq (1-\epsilon)\sqrt{2\log(p)}\}\right) \geq \frac{\{\sum_{k=1}^{p-L_p+1} \mathbb{P}(A_k)\}^2}{\sum_{i=1}^{p-L_p+1} \sum_{j=1}^{p-L_p+1} \mathbb{P}(A_i \cap A_j)}.$$

Note that

$$\begin{aligned} \sum_{i=1}^{p-L_p+1} \sum_{j=1}^{p-L_p+1} \mathbb{P}(A_i \cap A_j) &= \sum_{i=1}^{p-L_p+1} \mathbb{P}(A_i) + \sum_{\substack{i \neq j \\ 1 \leq i, j \leq p-L_p+1}} \mathbb{P}(A_i \cap A_j) \\ &= \sum_{i=1}^{p-L_p+1} \mathbb{P}(A_i) + \sum_{|i-j| \leq M_p+L_p} \mathbb{P}(A_i \cap A_j) + \sum_{|i-j| > M_p+L_p} \mathbb{P}(A_i \cap A_j) \\ &= \sum_{i=1}^{p-L_p+1} \mathbb{P}(A_i) + \sum_{|i-j| \leq M_p+L_p} \mathbb{P}(A_i \cap A_j) + \sum_{|i-j| > M_p+L_p} \mathbb{P}(A_i)\mathbb{P}(A_j) \\ &\leq (M_p + L_p + 1) \sum_{i=1}^{p-L_p+1} \mathbb{P}(A_i) + \sum_{|i-j| > M_p+L_p} \mathbb{P}(A_i)\mathbb{P}(A_j), \end{aligned}$$

then by condition (C), we get

$$\begin{aligned} &\frac{\{\sum_{k=1}^{p-L_p+1} \mathbb{P}(A_k)\}^2}{\sum_{i=1}^{p-L_p+1} \sum_{j=1}^{p-L_p+1} \mathbb{P}(A_i \cap A_j)} \\ &\geq \frac{\{\sum_{k=1}^{p-L_p+1} \mathbb{P}(A_k)\}^2}{(M_p + L_p + 1) \sum_{i=1}^{p-L_p+1} \mathbb{P}(A_i) + \sum_{|i-j| > M_p+L_p} \mathbb{P}(A_i)\mathbb{P}(A_j)} \\ &\geq 1 - \frac{(M_p + L_p + 1) \sum_{i=1}^{p-L_p+1} \mathbb{P}(A_i)}{(M_p + L_p + 1) \sum_{i=1}^{p-L_p+1} \mathbb{P}(A_i) + \sum_{|i-j| > M_p+L_p} \mathbb{P}(A_i)\mathbb{P}(A_j)} \\ &\geq 1 - \frac{(M_p + L_p + 1) \sum_{i=1}^{p-L_p+1} \mathbb{P}(A_i)}{\{\sum_{k=1}^{p-L_p+1} \mathbb{P}(A_k)\}^2} \\ &\geq 1 - \frac{M_p + L_p + 1}{\sum_{k=1}^{p-L_p+1} \mathbb{P}(A_k)}. \end{aligned}$$

By condition (A) and (B), using Lemma 1, there exists constant  $c_1, c_2 > 0$  such that

$$\sum_{k=1}^{p-L_p+1} \mathbb{P}(A_k) \geq \mathbb{P}[1 - \Phi\{(1-\epsilon)\sqrt{2\log(p)}\}] \exp\left\{\frac{2^{\frac{3}{2}}(1-\epsilon)^3(\log(p))^{\frac{3}{2}}}{\sqrt{L}}c_1\right\}c_2$$

Then, using Lemma 2, we have

$$\begin{aligned} \sum_{k=1}^{p-L_p+1} \mathbb{P}(A_k) &\geq \frac{p(1-\epsilon)\sqrt{2\log(p)}}{1+2(1-\epsilon)^2\log(p)} \exp\left\{\frac{2^{\frac{3}{2}}(1-\epsilon)^3(\log(p))^{\frac{3}{2}}}{\sqrt{L}}c_1\right\}c_2 \\ &\geq \frac{c_2}{4(1-\epsilon)} \exp\left\{\log(p)(2\epsilon-\epsilon^2+2^{\frac{3}{2}}c_1(1-\epsilon)^3\sqrt{\frac{\log(p)}{L_p}})-\frac{1}{2}\log(\log(p))\right\}. \end{aligned}$$

Hence by condition (B) and (C),

$$\frac{\sum_{k=1}^{p-L_p+1} \mathbb{P}(A_k)}{M_p + L_p + 1} \geq \frac{c_2}{4(1-\epsilon)} \exp\left[\log(p)\left\{2\epsilon-\epsilon^2+2^{\frac{3}{2}}c_1(1-\epsilon)^3\sqrt{\frac{\log(p)}{L_p}}\right\}-\frac{1}{2}\log(\log(p))-\log(M_p+L_p+1)\right] \rightarrow \infty.$$

This indicates that

$$\mathbb{P}\left(\max_{|I|=L_p} Q(I) < (1-\epsilon)\sqrt{2\log(p)}\right) \rightarrow 0 \quad (2)$$

Combine (1) and (2), we get

$$\mathbb{P}\left(\left|\frac{\max_{|I|=L_p} Q(I)}{\sqrt{2\log(p)}} - 1\right| > \epsilon\right) \rightarrow 0.$$

For the arbitrary of  $\epsilon$ , we complete the proof.  $\square$

We then prove the result of multi-length scan, which is the Theorem 1 in the paper.

**Theorem 1** *If the following conditions (A)-(C) hold,*

(A)  $\max_{|I|=L_{\max}} \|\lambda_I\|_{\infty} \leq K_0$ , where  $K_0$  is a constant,

(B)  $\frac{L_{\min}}{\log(p)} \rightarrow \infty$  and  $\frac{\log(L_{\max})}{\log(p)} \rightarrow 0$ ,

(C)  $\{U_i\}_{i=1}^p$  is  $M_p$ -dependent and  $\frac{\log(M_p)}{\log(p)} \rightarrow 0$ ,

then

$$\frac{\max_{L_{\min} \leq |I| \leq L_{\max}} Q(I)}{\sqrt{2\log(p)}} \xrightarrow{p} 1.$$

**Proof** For any  $\epsilon > 0$ ,

$$\begin{aligned} &\mathbb{P}\left(\left|\frac{\max_{L_{\min} \leq |I| \leq L_{\max}} Q(I)}{\sqrt{2\log(p)}} - 1\right| \geq \epsilon\right) \\ &= \mathbb{P}\left(\max_{L_{\min} \leq |I| \leq L_{\max}} Q(I) \geq (1+\epsilon)\sqrt{2\log(p)}\right) + \mathbb{P}\left(\max_{L_{\min} \leq |I| \leq L_{\max}} Q(I) \leq (1-\epsilon)\sqrt{2\log(p)}\right) \\ &\triangleq A_1(\epsilon) + A_2(\epsilon). \end{aligned}$$

Note that  $\max_{L_{\min} \leq |I| \leq L_{\max}} Q(I) \geq \max_{|I|=L_{\max}} Q(I)$ , by Lemma 4,

$$A_2(\epsilon) \leq \mathbb{P}\left(\max_{|I|=L_{\max}} Q(I) \leq (1 - \epsilon)\sqrt{2\log(p)}\right) = o(1). \quad (3)$$

For  $A_1(\epsilon)$ , by Boole's inequality,

$$A_1(\epsilon) \leq \sum_{L_{\min} \leq |I| \leq L_{\max}} \mathbb{P}\left(Q(I) \geq (1 + \epsilon)\sqrt{2\log(p)}\right).$$

For any  $I$  satisfies that  $L_{\min} \leq |I| \leq L_{\max}$ , by condition (B),

$$\frac{2(1 + \frac{\epsilon}{2})^2 \log(p) \|\lambda_I\|_{\infty}}{\|\lambda_I\|_2} \leq \frac{2K_0(1 + \frac{\epsilon}{2})^2 \log(p)}{\sqrt{L_{\min}}} = o(\sqrt{\log(p)}).$$

Hence, by Lemma 3,

$$A_1(\epsilon) \leq \sum_{L_{\min} \leq |I| \leq L_{\max}} \exp\{-(1 + \frac{\epsilon}{2})^2 \log(p)\} \leq \exp\{-(1 + \frac{\epsilon}{2})^2 \log(p) + \log(p) + \log(L_{\max})\} = o(1). \quad (4)$$

Using (3) and (4), we have

$$\mathbb{P}\left(\left|\frac{\max_{L_{\min} \leq |I| \leq L_{\max}} Q(I)}{\sqrt{2\log(p)}} - 1\right| \geq \epsilon\right) = o(1).$$

For the arbitrary of  $\epsilon$ , we complete the proof.  $\square$

Assume  $h(p, L_{\min}, L_{\max}, \alpha)$  is the  $(1 - \alpha)$ th quantile of  $Q_{\max}$ , that is,

$$\mathbb{P}(Q_{\max} > h(p, L_{\min}, L_{\max}, \alpha)) = \alpha.$$

Hence  $h(p, L_{\min}, L_{\max}, \alpha)$  is the threshold that control the family-wise error rate at  $\alpha$  level. By Theorem 1, for  $p$  sufficiently large, we have  $0.99\sqrt{2\log(p)} \leq h(p, L_{\min}, L_{\max}, \alpha) \leq 1.01\sqrt{2\log(p)}$ . Next we give a more accurate upper bound of  $h(p, L_{\min}, L_{\max}, \alpha)$ .

**Proposition 2** *If condition (A) and (B) hold, for  $p$  sufficiently large,*

$$h(p, L_{\min}, L_{\max}, \alpha) \leq \sqrt{2[\log\{p(L_{\max} - L_{\min})\} - \log(\alpha)]} + \frac{\sqrt{2}[\log\{p(L_{\max} - L_{\min})\} - \log(\alpha)]}{\{L_{\min} \log(p)\}^{\frac{1}{4}}}.$$

**Proof** Let  $\tilde{h}(p, \alpha) = \sqrt{2[\log\{p(L_{\max} - L_{\min})\} - \log(\alpha)]} + \frac{\sqrt{2}[\log\{p(L_{\max} - L_{\min})\} - \log(\alpha)]}{\{L_{\min} \log(p)\}^{\frac{1}{4}}}$ . For any  $I$  satisfies that  $L_{\min} \leq |I| \leq L_{\max}$ ,

$$\frac{2\|\lambda_I\|_{\infty}[\log\{p(L_{\max} - L_{\min})\} - \log(\alpha)]}{\sqrt{2}\|\lambda_I\|_2} = O\left(\frac{\sqrt{2}[\log\{p(L_{\max} - L_{\min})\} - \log(\alpha)]}{\sqrt{|I|}}\right).$$

Note that  $\frac{\log(p)}{|I|} \leq \frac{\log(p)}{L_{\min}} = o(1)$ , then for sufficiently large  $p$ ,

$$\frac{2\|\lambda_I\|_{\infty}[\log\{p(L_{\max} - L_{\min})\} - \log(\alpha)]}{\sqrt{2}\|\lambda_I\|_2} \leq \frac{\sqrt{2}[\log\{p(L_{\max} - L_{\min})\} - \log(\alpha)]}{(L_{\min} \log(p))^{\frac{1}{4}}}.$$

Hence, by Lemma 3,

$$\mathbb{P}(Q_{\max} > \tilde{h}(p, \alpha)) \leq \sum_{L_{\min} \leq |I| \leq L_{\max}} \exp(-\log\{p(L_{\max} - L_{\min})\} - \log(\alpha)) \leq \alpha.$$

Thus  $h(p, L_{\min}, L_{\max}, \alpha) \leq \tilde{h}(p, \alpha)$  and we complete the proof.  $\square$

By Theorem 1 and Proposition 2, for  $p$  sufficiently large,

$$0.99\sqrt{2\log(p)} \leq h(p, L_{\min}, L_{\max}, \alpha) \leq \sqrt{2[\log\{p(L_{\max} - L_{\min})\} - \log(\alpha)]} + \frac{\sqrt{2}[\log\{p(L_{\max} - L_{\min})\} - \log(\alpha)]}{\{L_{\min} \log(p)\}^{\frac{1}{4}}}.$$

## 1.2 Consistency of Signal Region Detection

In this section, we show the results of power analysis. We first proof the proposed Q-SCAN procedure could consistently select a signal region that overlaps with the true signal region. Let  $\boldsymbol{\mu}_I = \{\mu_i\}_{i \in I}$  for any region  $I$ . Assume  $I^*$  is the true signal region with  $\boldsymbol{\mu}_{I^*} \neq 0$  and  $L_{\min} \leq |I^*| \leq L_{\max}$ .

**Theorem 3** Assume condition (A)-(C) and the following condition (D) hold,

$$(D) \quad \frac{\|\boldsymbol{\mu}_{I^*}\|_2^2}{\|\boldsymbol{\lambda}_{I^*}\|_2} \geq 2(1 + \epsilon_0)\sqrt{\log(p)} \text{ for some constant } \epsilon_0 > 0,$$

then,

$$\mathbb{P}(Q(I^*) > h(p, L_{\min}, L_{\max}, \alpha)) \rightarrow 1.$$

**Proof**

$$\begin{aligned} \mathbb{P}(Q(I^*) \leq h(p, L_{\min}, L_{\max}, \alpha)) &= \mathbb{P}\left(\sum_{i \in I^*} U_i^2 - \|\boldsymbol{\lambda}_{I^*}\|_1 \leq \sqrt{2}\|\boldsymbol{\lambda}_{I^*}\|_2 h(p, L_{\min}, L_{\max}, \alpha)\right) \\ &= \mathbb{P}\left(\sum_{i \in I^*} U_i^2 - \|\boldsymbol{\lambda}_{I^*}\|_1 - \|\boldsymbol{\mu}_{I^*}\|_2^2 \leq \sqrt{2}\|\boldsymbol{\lambda}_{I^*}\|_2 h(p, L_{\min}, L_{\max}, \alpha) - \|\boldsymbol{\mu}_{I^*}\|_2^2\right) \\ &\leq \mathbb{P}\left(\left|\sum_{i \in I^*} U_i^2 - \|\boldsymbol{\lambda}_{I^*}\|_1 - \|\boldsymbol{\mu}_{I^*}\|_2^2\right| \geq \|\boldsymbol{\mu}_{I^*}\|_2^2 - \sqrt{2}\|\boldsymbol{\lambda}_{I^*}\|_2 h(p, L_{\min}, L_{\max}, \alpha)\right). \end{aligned}$$

Assume  $\boldsymbol{\Omega}_{I^*} \boldsymbol{\Sigma}_{I^*} \boldsymbol{\Omega}_{I^*}^T = \text{diag}(\boldsymbol{\lambda}_{I^*})$  is the SVD of  $\boldsymbol{\Sigma}_{I^*}$  where  $\boldsymbol{\Omega}_{I^*}$  is an orthogonal matrix. Let  $\tilde{\boldsymbol{U}}_{I^*} = \boldsymbol{\Omega}_{I^*} \boldsymbol{U}_{I^*}$  and then  $\tilde{\boldsymbol{U}}_{I^*} \sim N(\tilde{\boldsymbol{\mu}}_{I^*}, \text{diag}(\boldsymbol{\lambda}_{I^*}))$  where  $\tilde{\boldsymbol{\mu}}_{I^*} = \boldsymbol{\Omega}_{I^*} \boldsymbol{\mu}_{I^*}$ . Note that  $\sum_{i \in I^*} U_i^2 = \sum_{i \in I^*} \tilde{U}_i^2$  and  $\sum_{i \in I^*} \mu_i^2 = \sum_{i \in I^*} \tilde{\mu}_i^2$ , then

$$\text{Var}\left(\sum_{i \in I^*} U_i^2\right) = \text{Var}\left(\sum_{i \in I^*} \tilde{U}_i^2\right) = \sum_{i \in I^*} 4\lambda_i \tilde{\mu}_i^2 + 2\lambda_i^2 \leq 4\|\boldsymbol{\lambda}_{I^*}\|_{\infty} \|\boldsymbol{\mu}_{I^*}\|_2^2 + 2\|\boldsymbol{\lambda}_{I^*}\|_2^2.$$

Using condition (D) and Theorem 1, for  $p$  sufficiently large,

$$\frac{\sqrt{2}\|\boldsymbol{\lambda}_{I^*}\|_2 h(p, L_{\min}, L_{\max}, \alpha)}{\|\boldsymbol{\mu}_{I^*}\|_2^2} \leq \frac{h(p, L_{\min}, L_{\max}, \alpha)}{\sqrt{2}(1 + \epsilon)\sqrt{\log(p)}} \leq 1 - \frac{\epsilon_0}{2}.$$

Hence, by Chebyshev's inequality,

$$\begin{aligned}
\mathbb{P}(Q(I^*) \leq h(p, L_{\min}, L_{\max}, \alpha)) &\leq \frac{16\|\boldsymbol{\lambda}_{I^*}\|_{\infty}\|\boldsymbol{\mu}_{I^*}\|_2^2 + 8\|\boldsymbol{\lambda}_{I^*}\|_2^2}{\epsilon_0^2\|\boldsymbol{\mu}_{I^*}\|_2^4} \\
&\leq \frac{16\|\boldsymbol{\lambda}_{I^*}\|_{\infty}}{\epsilon_0^2\|\boldsymbol{\mu}_{I^*}\|_2^2} + \frac{2}{\epsilon_0^2(1+\epsilon_0)^2\log(p)} \\
&\leq \frac{8}{\epsilon_0^2(1+\epsilon_0)\sqrt{\log(p)}} + \frac{1}{\epsilon_0^2(1+\epsilon_0)^2\log(p)} = o(1).
\end{aligned}$$

Thus we complete the proof.  $\square$

For any region  $I_1$  and  $I_2$ , define the Jaccard index between  $I_1$  and  $I_2$  as  $J(I_1, I_2) = \frac{|I_1 \cap I_2|}{|I_1 \cup I_2|}$ . It is obvious that  $0 \leq J(I_1, I_2) \leq 1$ . We define region  $I^*$  is consistently detected if for some  $\eta_p = o(1)$ , there exists  $\hat{I} \in \hat{\mathcal{I}}$  such that

$$\mathbb{P}(J(\hat{I}, I^*) \geq 1 - \eta_p) \rightarrow 1.$$

Next we show that the proposed Q-SCAN could consistently detect the true signal region.

**Theorem 4** Assume condition (A)-(D) and the following condition (E) hold,

$$(E) \inf_{I \subseteq I^*} \frac{\log(\|\boldsymbol{\mu}_{I^*}\|_2^2) - \log(\|\boldsymbol{\mu}_I\|_2^2)}{\log(\|\boldsymbol{\lambda}_{I^*}\|_2) - \log(\|\boldsymbol{\lambda}_I\|_2)} > 1,$$

then

$$\mathbb{P}(J(\hat{I}, I^*) \geq 1 - \eta_p) \rightarrow 1,$$

where  $\left\{\frac{\log(L_{\max})}{\log(p)}\right\}^{\frac{1}{4}} \ll \eta_p \ll 1$ .

**Proof**

$$\begin{aligned}
\mathbb{P}(J(\hat{I}, I^*) \geq 1 - \eta_p) &= \mathbb{P}(J(\hat{I}, I^*) < 1 - \eta_p, \hat{I} \cap I^* = \emptyset) + \mathbb{P}(J(\hat{I}, I^*) < 1 - \eta_p, \hat{I} \cap I^* \neq \emptyset) \\
&\leq \mathbb{P}\left(\sup_{I \cap I^* = \emptyset} Q(I) > Q(I^*)\right) + \mathbb{P}(J(\hat{I}, I^*) < 1 - \eta_p, \hat{I} \cap I^* \neq \emptyset) \\
&\leq \mathbb{P}\left(\sup_{I \cap I^* \neq \emptyset} Q(I) > (1 + \frac{\epsilon}{4})\sqrt{2\log(p)}\right) + \mathbb{P}(Q(I^*) \leq (1 + \frac{\epsilon_0}{4})\sqrt{2\log(p)}) \\
&\quad + \mathbb{P}(J(\hat{I}, I^*) < 1 - \eta_p, \hat{I} \cap I^* \neq \emptyset).
\end{aligned}$$

For the first part, by Theorem 1,

$$\mathbb{P}\left(\sup_{I \cap I^* \neq \emptyset} Q(I) > (1 + \frac{\epsilon}{4})\sqrt{2\log(p)}\right) = o(1). \quad (5)$$

For the second part, by the same approach discussed in Theorem 3,

$$\mathbb{P}(Q(I^*) \leq (1 + \frac{\epsilon_0}{4})\sqrt{2\log(p)}) = o(1). \quad (6)$$

We now consider the third part. Note that

$$J(\hat{I}, I^*) = \frac{|\hat{I} \cap I^*|}{|\hat{I} \cup I^*|} = \frac{|I^*| - |I^* \setminus \hat{I}|}{|I^*| + |\hat{I} \setminus I^*|},$$



then  $J(\hat{I}, I^*) < 1 - \eta_p$  implies that  $|\hat{I} \setminus I^*| > \frac{\eta_p}{2} |I^*|$  or  $|I^* \setminus \hat{I}| > \frac{\eta_p}{2} |I^*|$ . Thus we get

$$\begin{aligned}
& \mathbb{P}(J(\hat{I}, I^*) < 1 - \eta_p, \hat{I} \cap I^* \neq \emptyset) \\
& \leq \mathbb{P}\left(\sup_{\substack{I \cap I^* \neq \emptyset \\ J(I, I^*) < 1 - \eta_p}} Q(I) - Q(I^*) > 0\right) \\
& = \mathbb{P}\left(\bigcup_{\substack{I \cap I^* \neq \emptyset \\ J(I, I^*) < 1 - \eta_p}} Q(I) - Q(I^*) > 0\right) \\
& \leq \mathbb{P}\left(\bigcup_{\substack{I \cap I^* \neq \emptyset \\ |I \setminus I^*| > \frac{\eta_p}{2} |I^*|}} \{Q(I) - Q(I^*) > 0\}\right) + \mathbb{P}\left(\bigcup_{\substack{I \cap I^* \neq \emptyset \\ |I^* \setminus I| > \frac{\eta_p}{2} |I^*|}} \{Q(I) - Q(I^*) > 0\}\right) \\
& \leq \sum_{\substack{I \cap I^* \neq \emptyset \\ |I \setminus I^*| > \frac{\eta_p}{2} |I^*|}} \mathbb{P}(Q(I) - Q(I^*) > 0) + \sum_{\substack{I \cap I^* \neq \emptyset \\ |I^* \setminus I| > \frac{\eta_p}{2} |I^*|}} \mathbb{P}(Q(I) - Q(I^*) > 0) \tag{7}
\end{aligned}$$

Let  $\tilde{U}_i = U_i - \mu_i$ , for any  $I \cap I^* \neq \emptyset$ , we have

$$\begin{aligned}
Q(I) - Q(I^*) &= \frac{\sum_{i \in I} U_i^2 - \|\boldsymbol{\lambda}_I\|_1}{\sqrt{2} \|\boldsymbol{\lambda}_I\|_2} - \frac{\sum_{i \in I^*} U_i^2 - \|\boldsymbol{\lambda}_{I^*}\|_1}{\sqrt{2} \|\boldsymbol{\lambda}_{I^*}\|_2} \\
&= \frac{\sum_{i \in I} (\tilde{U}_i + \mu_i)^2 - \|\boldsymbol{\lambda}_I\|_1}{\sqrt{2} \|\boldsymbol{\lambda}_I\|_2} - \frac{\sum_{i \in I^*} (\tilde{U}_i + \mu_i)^2 - \|\boldsymbol{\lambda}_{I^*}\|_1}{\sqrt{2} \|\boldsymbol{\lambda}_{I^*}\|_2} \\
&= \frac{\sum_{i \in I \setminus I^*} \tilde{U}_i^2 - \|\boldsymbol{\lambda}_{I \setminus I^*}\|_1}{\sqrt{2} \|\boldsymbol{\lambda}_I\|_2} + \left(1 - \frac{\|\boldsymbol{\lambda}_I\|_2}{\|\boldsymbol{\lambda}_{I^*}\|_2}\right) \frac{\sum_{i \in I \cap I^*} \tilde{U}_i^2 - \|\boldsymbol{\lambda}_{I \cap I^*}\|_1}{\sqrt{2} \|\boldsymbol{\lambda}_I\|_2} \\
&\quad + \frac{2 \sum_{i \in I \cap I^*} \mu_i \tilde{U}_i}{\sqrt{2} \|\boldsymbol{\lambda}_I\|_2} \left(1 - \frac{\|\boldsymbol{\lambda}_I\|_2}{\|\boldsymbol{\lambda}_{I^*}\|_2}\right) - \frac{2 \sum_{i \in I^* \setminus I} \mu_i \tilde{U}_i}{\sqrt{2} \|\boldsymbol{\lambda}_{I^*}\|_2} - \frac{\sum_{i \in I^* \setminus I} \tilde{U}_i^2 - \|\boldsymbol{\lambda}_{I^* \setminus I}\|_1}{\sqrt{2} \|\boldsymbol{\lambda}_{I^*}\|_2} \\
&\quad + \frac{\|\boldsymbol{\mu}_{I \cap I^*}\|_2^2}{\sqrt{2} \|\boldsymbol{\lambda}_I\|_2} - \frac{\|\boldsymbol{\mu}_{I^*}\|_2^2}{\sqrt{2} \|\boldsymbol{\lambda}_{I^*}\|_2} \tag{8}
\end{aligned}$$

Assume  $\delta = \inf_{I \subsetneq I^*} \frac{\log(\|\boldsymbol{\mu}_{I^*}\|_2^2) - \log(\|\boldsymbol{\mu}_I\|_2^2)}{\log(\|\boldsymbol{\lambda}_{I^*}\|_2) - \log(\|\boldsymbol{\lambda}_I\|_2)} - 1$ , then by condition (E), there exists  $\delta > 0$  and for any  $I$ ,

$$\frac{\|\boldsymbol{\mu}_{I^*}\|_2^2}{\|\boldsymbol{\lambda}_{I^*}\|_2} - \frac{\|\boldsymbol{\mu}_{I \cap I^*}\|_2^2}{\|\boldsymbol{\lambda}_I\|_2} \geq \frac{\|\boldsymbol{\mu}_{I^*}\|_2^2}{\|\boldsymbol{\lambda}_{I^*}\|_2} \left(1 - \frac{\|\boldsymbol{\lambda}_{I \cap I^*}\|_2^{1+\delta}}{\|\boldsymbol{\lambda}_I\|_2 \|\boldsymbol{\lambda}_{I^*}\|_2^\delta}\right).$$

Then by (8), we have

$$\mathbb{P}(Q(I) - Q(I^*) > 0) \leq \sum_{i=1}^5 \mathbb{P}(A_i(I)),$$

where

$$\begin{aligned}
A_1(I) &= \left\{ \frac{\sum_{i \in I \setminus I^*} \tilde{U}_i^2 - \|\lambda_{I \setminus I^*}\|_1}{\sqrt{2}\|\lambda_I\|_2} > \frac{\|\mu_{I^*}\|_2^2}{5\sqrt{2}\|\lambda_{I^*}\|_2} \left(1 - \frac{\|\lambda_{I \cap I^*}\|_2^{1+\delta}}{\|\lambda_I\|_2 \|\lambda_{I^*}\|_2^\delta} \right) \right\}, \\
A_2(I) &= \left\{ \left(1 - \frac{\|\lambda_I\|_2}{\|\lambda_{I^*}\|_2}\right) \frac{\sum_{i \in I \cap I^*} \tilde{U}_i^2 - \|\lambda_{I \cap I^*}\|_1}{\sqrt{2}\|\lambda_I\|_2} > \frac{\|\mu_{I^*}\|_2^2}{5\sqrt{2}\|\lambda_{I^*}\|_2} \left(1 - \frac{\|\lambda_{I \cap I^*}\|_2^{1+\delta}}{\|\lambda_I\|_2 \|\lambda_{I^*}\|_2^\delta} \right) \right\}, \\
A_3(I) &= \left\{ -\frac{\sum_{i \in I^* \setminus I} \tilde{U}_i^2 - \|\lambda_{I^* \setminus I}\|_1}{\sqrt{2}\|\lambda_{I^*}\|_2} > \frac{\|\mu_{I^*}\|_2^2}{5\sqrt{2}\|\lambda_{I^*}\|_2} \left(1 - \frac{\|\lambda_{I \cap I^*}\|_2^{1+\delta}}{\|\lambda_I\|_2 \|\lambda_{I^*}\|_2^\delta} \right) \right\}, \\
A_4(I) &= \left\{ \frac{2 \sum_{i \in I \cap I^*} \mu_i \tilde{U}_i}{\sqrt{2}\|\lambda_I\|_2} \left(1 - \frac{\|\lambda_I\|_2}{\|\lambda_{I^*}\|_2}\right) > \frac{\|\mu_{I^*}\|_2^2}{5\sqrt{2}\|\lambda_{I^*}\|_2} \left(1 - \frac{\|\lambda_{I \cap I^*}\|_2^{1+\delta}}{\|\lambda_I\|_2 \|\lambda_{I^*}\|_2^\delta} \right) \right\}, \\
A_5(I) &= \left\{ -\frac{2 \sum_{i \in I^* \setminus I} \mu_i \tilde{U}_i}{\sqrt{2}\|\lambda_{I^*}\|_2} > \frac{\|\mu_{I^*}\|_2^2}{5\sqrt{2}\|\lambda_{I^*}\|_2} \left(1 - \frac{\|\lambda_{I \cap I^*}\|_2^{1+\delta}}{\|\lambda_I\|_2 \|\lambda_{I^*}\|_2^\delta} \right) \right\}.
\end{aligned}$$

We first consider  $A_1(I)$ . When  $|I \setminus I^*| \geq \frac{\eta_p |I^*|}{2}$ ,

$$\frac{|I \setminus I^*|}{|I|} = \frac{|I \setminus I^*|}{|I \setminus I^*| + |I \cap I^*|} \geq \frac{\frac{\eta_p}{2} |I^*|}{\frac{\eta_p}{2} |I^*| + |I^*|} = \frac{\eta_p}{2 + \eta_p} \geq \frac{\eta_p}{3},$$

then we have

$$\frac{\|\lambda_I\|_2^2 - \|\lambda_{I \cap I^*}\|_2^2}{\|\lambda_I\|_2^2} \geq \frac{\|\lambda_{I \setminus I^*}\|_2^2}{K_0^2 |I|} \geq \frac{\|\lambda_{I \setminus I^*}\|_1^2}{K_0^2 |I| \times |I \setminus I^*|} \geq \frac{c^2 |I \setminus I^*|}{K_0^2 |I|} \geq \frac{c^2 \eta_p}{3K_0^2},$$

and by the same approach, we get  $\frac{\|\lambda_I\|_2^2 - \|\lambda_{I \cap I^*}\|_2^2}{\|\lambda_{I^*}\|_2^2} \geq \frac{c^2 \eta_p}{2K_0^2}$ . It follows that

$$\frac{\|\lambda_I\|_2^2 - \|\lambda_{I \cap I^*}\|_2^2}{\|\lambda_I\|_2 (\|\lambda_{I^*}\|_2 + \|\lambda_I\|_2)} \geq \frac{\|\lambda_I\|_2^2 - \|\lambda_{I \cap I^*}\|_2^2}{\frac{1}{2}\|\lambda_I\|_2^2 + \frac{3}{2}\|\lambda_{I^*}\|_2^2} \geq \frac{2c^2 \eta_p}{9K_0^2},$$

and hence

$$\begin{aligned}
\frac{\|\mu_{I^*}\|_2^2 (\|\lambda_I\|_2 \|\lambda_{I^*}\|_2^\delta - \|\lambda_{I \cap I^*}\|_2^{1+\delta})}{\|\lambda_{I^*}\|_2^{1+\delta}} &\geq \frac{\|\mu_{I^*}\|_2^2 (\|\lambda_I\|_2 - \|\lambda_{I \cap I^*}\|_2)}{\|\lambda_{I^*}\|_2} \\
&= \frac{\|\mu_{I^*}\|_2^2 (\|\lambda_I\|_2^2 - \|\lambda_{I \cap I^*}\|_2^2)}{(\|\lambda_{I^*}\|_2 + \|\lambda_{I \cap I^*}\|_2) \|\lambda_{I^*}\|_2} \\
&\geq \frac{\|\mu_{I^*}\|_2^2 (\|\lambda_I\|_2^2 - \|\lambda_{I \cap I^*}\|_2^2)}{(\|\lambda_I\|_2 + \|\lambda_{I^*}\|_2) \|\lambda_{I^*}\|_2} \\
&\geq \frac{2c^2 \eta_p \|\mu_{I^*}\|_2^2}{9K_0^2}.
\end{aligned}$$

On the other hand,

$$\frac{\|\lambda_I\|_2^2 - \|\lambda_{I \cap I^*}\|_2^2}{(\|\lambda_I\|_2 + \|\lambda_{I^*}\|_2) \|\lambda_{I^*}\|_2} \geq \frac{\|\lambda_{I^* \setminus I}\|_2}{\|\lambda_{I^*}\|_2} \times \sqrt{\frac{\|\lambda_I\|_2^2 - \|\lambda_{I \cap I^*}\|_2^2}{(\|\lambda_I\|_2 + \|\lambda_{I^*}\|_2)^2}} \geq \frac{c \eta_p \|\lambda_{I^* \setminus I}\|_2}{4K_0 \|\lambda_{I^*}\|_2}$$

and thus

$$\frac{\|\mu_{I^*}\|_2^2 (\|\lambda_I\|_2 \|\lambda_{I^*}\|_2^\delta - \|\lambda_{I \cap I^*}\|_2^{1+\delta})}{\|\lambda_{I^*}\|_2^{1+\delta}} \geq \frac{\|\mu_{I^*}\|_2^2}{\|\lambda_{I^*}\|_2} \times \frac{c \eta_p \|\lambda_{I^* \setminus I}\|_2}{4K_0}.$$

Note that  $2\|\boldsymbol{\lambda}_{I \setminus I^*}\|_2 \sqrt{3 \log(L_{\max})} = o(\|\boldsymbol{\lambda}_{I^* \setminus I}\|_2 \eta_p \sqrt{\log(p)})$  and  $6\|\boldsymbol{\lambda}_{I \setminus I^*}\|_\infty \log(L_{\max}) = o(\eta_p \|\boldsymbol{\mu}_{I^*}\|_2^2)$ , by Lemma 3, we have  $\mathbb{P}(A_1(I)) \leq 1/L_{\max}^3$  and thus

$$\sum_{\substack{I \cap I^* \neq \emptyset \\ |I \setminus I^*| > \frac{\eta_p}{2} |I^*|}} \mathbb{P}(A_1(I)) \leq \frac{2L_{\max}^2}{L_{\max}^3} = \frac{2}{L_{\max}} = o(1). \quad (9)$$

When  $|I^* \setminus I| \geq \frac{\eta_p}{2} |I^*|$ , we have

$$\frac{\|\boldsymbol{\lambda}_{I \cap I^*}\|_2^2}{\|\boldsymbol{\lambda}_{I^*}\|_2^2} \leq \frac{\|\boldsymbol{\lambda}_{I^*}\|_2^2 - \|\boldsymbol{\lambda}_{I^* \setminus I}\|_2^2}{\|\boldsymbol{\lambda}_{I^*}\|_2^2} \leq 1 - \frac{c^2 |I^* \setminus I|}{K_0^2 |I^*|} \leq 1 - \frac{c^2 \eta_p}{2K_0^2},$$

and then

$$1 - \left( \frac{\|\boldsymbol{\lambda}_{I \cap I^*}\|_2}{\|\boldsymbol{\lambda}_{I^*}\|_2} \right)^\delta \geq 1 - \left( 1 - \frac{c^2 \eta_p}{2K_0^2} \right)^{\frac{\delta}{2}} \geq \frac{\delta c^2 \eta_p}{4K_0^2}.$$

Note that

$$\begin{aligned} \frac{\|\boldsymbol{\mu}_{I^*}\|_2^2 (\|\boldsymbol{\lambda}_I\|_2 \|\boldsymbol{\lambda}_{I^*}\|_2^\delta - \|\boldsymbol{\lambda}_{I \cap I^*}\|_2^{1+\delta})}{\|\boldsymbol{\lambda}_{I^*}\|_2^{1+\delta}} &\geq \frac{\|\boldsymbol{\mu}_{I^*}\|_2^2 \|\boldsymbol{\lambda}_I\|_2 (\|\boldsymbol{\lambda}_{I^*}\|_2^\delta - \|\boldsymbol{\lambda}_{I \cap I^*}\|_2^\delta)}{\|\boldsymbol{\lambda}_{I^*}\|_2^{1+\delta}} \\ &\geq \frac{\delta c^2 \eta_p \|\boldsymbol{\mu}_{I^*}\|_2^2 \|\boldsymbol{\lambda}_I\|_2}{2K_0^2 \|\boldsymbol{\lambda}_{I^*}\|_2} \\ &\geq \frac{\delta c^2 \eta_p \sqrt{\log(p)} \|\boldsymbol{\lambda}_I\|_2}{K_0^2}, \end{aligned}$$

and  $\|\boldsymbol{\lambda}_I\|_2 \sqrt{\log p} \geq c \sqrt{|I| \log(p)} \geq c \sqrt{L_{\min} \log(p)}$ , we have

$$2\|\boldsymbol{\lambda}_{I \setminus I^*}\|_2 \sqrt{3 \log(L_{\max})} + 6\|\boldsymbol{\lambda}_{I \setminus I^*}\|_\infty \log(L_{\max}) = o(\eta_p \sqrt{\log(p)} \|\boldsymbol{\lambda}_I\|_2).$$

Then by Lemma 3, we have  $\mathbb{P}(A_1(I)) \leq 1/L_{\max}^3$  and thus

$$\sum_{\substack{I^* \cap I \neq \emptyset \\ |I \setminus I^*| > \frac{\eta_p}{2} |I^*|}} \mathbb{P}(A_1(I)) \leq \frac{2L_{\max}^2}{L_{\max}^3} = \frac{2}{L_{\max}} = o(1). \quad (10)$$

Next we consider  $A_2(I)$ , when  $\|\boldsymbol{\lambda}_{I^*}\|_2 < \|\boldsymbol{\lambda}_I\|_2$ ,

$$\frac{\|\boldsymbol{\mu}_{I^*}\|_2^2 (\|\boldsymbol{\lambda}_I\|_2 \|\boldsymbol{\lambda}_{I^*}\|_2^\delta - \|\boldsymbol{\lambda}_{I \cap I^*}\|_2^{1+\delta})}{(\|\boldsymbol{\lambda}_I\|_2 - \|\boldsymbol{\lambda}_{I \cap I^*}\|_2) \|\boldsymbol{\lambda}_{I^*}\|_2^\delta} \geq \|\boldsymbol{\mu}_{I^*}\|_2^2 \geq 2\|\boldsymbol{\lambda}_{I^*}\|_2 \sqrt{\log(p)},$$

by Lemma 3,  $\mathbb{P}(A_2(I)) \leq \frac{1}{p}$ . When  $\|\boldsymbol{\lambda}_{I^*}\|_2 \geq \|\boldsymbol{\lambda}_I\|_2$ , let  $x = \|\boldsymbol{\lambda}_{I \cap I^*}\|_2 / \|\boldsymbol{\lambda}_{I^*}\|_2$ , we have

$$\frac{\|\boldsymbol{\lambda}_I\|_2 (\|\boldsymbol{\lambda}_{I^*}\|_2^\delta - \|\boldsymbol{\lambda}_{I \cap I^*}\|_2^\delta)}{(\|\boldsymbol{\lambda}_{I^*}\|_2 - \|\boldsymbol{\lambda}_{I \cap I^*}\|_2) \|\boldsymbol{\lambda}_{I^*}\|_2^\delta} = \frac{\|\boldsymbol{\lambda}_I\|_2}{\|\boldsymbol{\lambda}_{I^*}\|_2} \left( \frac{1 - x^\delta}{1 - x} \right) \geq \frac{\delta \|\boldsymbol{\lambda}_I\|_2}{\|\boldsymbol{\lambda}_{I^*}\|_2}.$$

It follows that

$$\begin{aligned}
& \frac{\|\mu_{I^*}\|_2^2 (\|\lambda_I\|_2 \|\lambda_{I^*}\|_2^\delta - \|\lambda_{I \cap I^*}\|_2^{1+\delta})}{\|\lambda_I\|_2 \|\lambda_{I^*}\|_2^{1+\delta}} \times \frac{\|\lambda_I\|_2 \|\lambda_{I^*}\|_2}{\|\lambda_{I^*}\|_2 - \|\lambda_I\|_2} \\
&= \frac{\|\mu_{I^*}\|_2^2 (\|\lambda_I\|_2 \|\lambda_{I^*}\|_2^\delta - \|\lambda_{I \cap I^*}\|_2^{1+\delta})}{(\|\lambda_{I^*}\|_2 - \|\lambda_I\|_2) \|\lambda_{I^*}\|_2^\delta} \\
&\geq \frac{\|\mu_{I^*}\|_2^2 \|\lambda_I\|_2 (\|\lambda_{I^*}\|_2^\delta - \|\lambda_{I \cap I^*}\|_2^\delta)}{(\|\lambda_{I^*}\|_2 - \|\lambda_{I \cap I^*}\|_2) \|\lambda_{I^*}\|_2^\delta} \\
&\geq \frac{\delta \|\mu_{I^*}\|_2^2 \|\lambda_I\|_2}{\|\lambda_{I^*}\|_2} \geq 2\delta \|\lambda_I\|_2 \sqrt{\log(p)}.
\end{aligned}$$

Note that  $2\|\lambda_{I \cap I^*}\|_2 \sqrt{3 \log(L_{\max})} + 6\|\lambda_{I \cap I^*}\|_\infty \log(L_{\max}) = o(\|\lambda_I\|_2 \sqrt{\log(p)})$ , by Lemma 3,  $\mathbb{P}(A_2(I)) \leq \frac{1}{L_{\max}^3}$ . Hence,

$$\sum_{I \cap I^* \neq \emptyset} \mathbb{P}(A_2(I)) = \sum_{\substack{I \cap I^* \neq \emptyset \\ \|\lambda_{I^*}\|_2 \geq \|\lambda_I\|_2}} \mathbb{P}(A_2(I)) + \sum_{\substack{I \cap I^* \neq \emptyset \\ \|\lambda_{I^*}\|_2 < \|\lambda_I\|_2}} \mathbb{P}(A_2(I)) \leq \frac{2}{L_{\max}} + \frac{2L_{\max}^2}{p} = o(1). \quad (11)$$

Then we consider  $A_3(I)$ , when  $|I \setminus I^*| \geq \frac{\eta_p}{2} |I^*|$ , by the former discussion, we have  $\frac{\|\lambda_I\|_2^2 - \|\lambda_{I \cap I^*}\|_2^2}{\|\lambda_I\|_2 (\|\lambda_{I^*}\|_2 + \|\lambda_I\|_2)} \geq \frac{c^2 \eta_p}{6K_0^2}$ . It follows that

$$\frac{\|\mu_{I^*}\|_2^2 (\|\lambda_I\|_2 \|\lambda_{I^*}\|_2^\delta - \|\lambda_{I \cap I^*}\|_2^{1+\delta})}{\|\lambda_I\|_2 \|\lambda_{I^*}\|_2^\delta} \geq \frac{\|\mu_{I^*}\|_2^2 (\|\lambda_I\|_2^2 - \|\lambda_{I \cap I^*}\|_2^2)}{\|\lambda_I\|_2 (\|\lambda_I\|_2 + \|\lambda_{I^*}\|_2)} \geq \frac{\eta_p \|\mu_{I^*}\|_2^2}{6K_0^2}.$$

Therefore  $\|\lambda_{I^* \setminus I}\|_2 \sqrt{3 \log(L_{\max})} \leq \|\lambda_{I^*}\|_2 \sqrt{3 \log(L_{\max})} = o(\eta_p \|\mu_{I^*}\|_2^2)$  and by Lemma 3, we get  $\mathbb{P}(A_3(I)) \leq \frac{1}{L_{\max}^3}$ . Hence,

$$\sum_{\substack{I \cap I^* \neq \emptyset \\ |I \setminus I^*| \geq \frac{\eta_p}{2} |I^*|}} \mathbb{P}(A_3(I)) \leq \frac{2}{L_{\max}} = o(1). \quad (12)$$

When  $|I^* \setminus I| \geq \frac{\eta_p}{2} |I^*|$ , by the former discussion, we have  $\frac{\|\lambda_{I \cap I^*}\|_2^2}{\|\lambda_{I^*}\|_2^2} \leq 1 - \frac{\eta_p}{2K_0^2}$ . It follows that

$$\begin{aligned}
\frac{\|\mu_{I^*}\|_2^2 (\|\lambda_I\|_2 \|\lambda_{I^*}\|_2^\delta - \|\lambda_{I \cap I^*}\|_2^{1+\delta})}{\|\lambda_I\|_2 \|\lambda_{I^*}\|_2^\delta} &\geq \frac{\|\mu_{I^*}\|_2^2 (\|\lambda_{I^*}\|_2^\delta - \|\lambda_{I \cap I^*}\|_2^\delta)}{\|\lambda_{I^*}\|_2^\delta} \\
&\geq \|\mu_{I^*}\|_2^2 \left\{ 1 - \left( 1 - \frac{c^2 \eta_p}{2K_0^2} \right)^{\frac{\delta}{2}} \right\} \geq \frac{c^2 \delta \eta_p \|\mu_{I^*}\|_2}{4K_0^2}.
\end{aligned}$$

Therefore  $\|\lambda_{I^* \setminus I}\|_2 \sqrt{3 \log(L_{\max})} \leq \|\lambda_{I^*}\|_2 \sqrt{3 \log(L_{\max})} = o(\eta_p \|\mu_{I^*}\|_2^2)$  and by Lemma 3, we  $\mathbb{P}(A_3(I)) \leq \frac{1}{L_{\max}^3}$ . Hence,

$$\sum_{\substack{I \cap I^* \neq \emptyset \\ |I^* \setminus I| \geq \frac{\eta_p}{2} |I^*|}} \mathbb{P}(A_3(I)) \leq \frac{2}{L_{\max}} = o(1). \quad (13)$$

We now consider  $A_4(I)$ .

$$\text{Var} \left\{ \frac{\sqrt{2} \sum_{i \in I \cap I^*} \mu_i \tilde{U}_i}{\|\lambda_I\|_2} \left( 1 - \frac{\|\lambda_I\|_2}{\|\lambda_{I^*}\|_2} \right) \right\} = \frac{2\mu_{I \cap I^*} \Sigma_{I \cap I^*} \mu_{I \cap I^*} (\|\lambda_{I^*}\|_2 - \|\lambda_I\|_2)^2}{\|\lambda_I\|_2^2 \|\lambda_{I^*}\|_2^2}$$

By condition (D) and (E),

$$\begin{aligned}
\kappa &= \frac{\frac{\|\mu_{I^*}\|_2^2(\|\lambda_I\|_2\|\lambda_{I^*}\|_2^\delta - \|\lambda_{I \cap I^*}\|_2^{1+\delta})}{\|\lambda_I\|_2\|\lambda_{I^*}\|_2^{1+\delta}}}{\frac{2\sqrt{\mu_{I \cap I^*}^T \Sigma_{I \cap I^*} \mu_{I \cap I^*}} \|\lambda_{I^*}\|_2 - \|\lambda_I\|_2}{\|\lambda_I\|_2\|\lambda_{I^*}\|_2}} \\
&= \frac{\frac{\|\mu_{I^*}\|_2^2(\|\lambda_I\|_2\|\lambda_{I^*}\|_2^\delta - \|\lambda_{I \cap I^*}\|_2^{1+\delta})}{2\sqrt{\mu_{I \cap I^*}^T \Sigma_{I \cap I^*} \mu_{I \cap I^*}} \|\lambda_{I^*}\|_2^\delta \|\lambda_{I^*}\|_2 - \|\lambda_I\|_2}{\frac{\|\mu_{I^*}\|_2^2(\|\lambda_I\|_2\|\lambda_{I^*}\|_2^\delta - \|\lambda_{I \cap I^*}\|_2^{1+\delta})}{2\sqrt{K_0}\|\mu_{I \cap I^*}\|_2 \|\lambda_{I^*}\|_2^{1+\delta} - \|\lambda_I\|_2\|\lambda_{I^*}\|_2^\delta}} \\
&\geq \frac{(\log(p))^{\frac{1}{4}}\|\lambda_{I^*}\|_2^{1+\frac{\delta}{2}}(\|\lambda_I\|_2 - \|\lambda_{I^*}\|_2)}{\sqrt{K_0}(\|\lambda_I\|_2 - \|\lambda_{I^*}\|_2)\|\lambda_{I^*}\|_2^{\frac{1}{2}+\frac{\delta}{2}}} = \frac{(\log(p))^{\frac{1}{4}}\|\lambda_{I^*}\|_2^{\frac{1}{2}}}{\sqrt{K_0}} \geq \frac{\sqrt{c}|I^*|^{\frac{1}{4}}(\log(p))^{\frac{1}{4}}}{\sqrt{K_0}} \geq \frac{\sqrt{\log(p)}}{\sqrt{K_0}}.
\end{aligned}$$

When  $\|\lambda_I\|_2 \geq \|\lambda_{I^*}\|_2$ , we have

$$\kappa \geq \frac{(\log(p))^{\frac{1}{4}}\|\lambda_{I^*}\|_2^{1+\frac{\delta}{2}}(\|\lambda_I\|_2 - \|\lambda_{I^*}\|_2)}{\sqrt{K_0}(\|\lambda_I\|_2 - \|\lambda_{I^*}\|_2)\|\lambda_{I^*}\|_2^{\frac{1}{2}+\frac{\delta}{2}}} = \frac{(\log(p))^{\frac{1}{4}}\|\lambda_{I^*}\|_2^{\frac{1}{2}}}{\sqrt{K_0}} \geq \frac{\sqrt{c}|I^*|^{\frac{1}{4}}(\log(p))^{\frac{1}{4}}}{\sqrt{K_0}} \geq \frac{\sqrt{\log(p)}}{\sqrt{K_0}}.$$

It is obviously that  $\sqrt{4\log(L_{\max}) + 2\log(\log(p))} = o(\sqrt{\log(p)})$ , then

$$\mathbb{P}(A_4(I)) \leq \mathbb{P}\left(\frac{\frac{\sqrt{2}\sum_{i \in I \cap I^*} \mu_i \tilde{U}_i (1 - \frac{\|\lambda_I\|_2}{\|\lambda_{I^*}\|_2})}{\sqrt{\frac{4\mu_{I \cap I^*}^T \Sigma_{I \cap I^*} \mu_{I \cap I^*} (\|\lambda_{I^*}\|_2 - \|\lambda_I\|_2^2)^2}{\|\lambda_I\|_2^2 \|\lambda_{I^*}\|_2^2}}} > \sqrt{4\log(L_{\max}) + 2\log(\log(p))}\right).$$

Hence, by Lemma 2,

$$\mathbb{P}(A_4(I)) \leq \frac{1}{\sqrt{4\log(L_{\max}) + 2\log(\log(p))}(L_{\max}^2 \log(p))} \leq \frac{1}{L_{\max}^2 \log(p)}.$$

When  $\|\lambda_{I^*}\|_2 \geq \|\lambda_I\|_2$ , we have

$$\kappa \geq \frac{(\log(p))^{\frac{1}{4}}\|\lambda_{I^*}\|_2^{1-\frac{\delta}{2}}\|\lambda_{I^*}\|_2^{1-\frac{\delta}{2}}\|\lambda_I\|_2^{\frac{1}{2}-\frac{\delta}{2}}(\|\lambda_{I^*}\|_2^\delta - \|\lambda_I\|_2^\delta)}{\sqrt{K_0}(\|\lambda_{I^*}\|_2 - \|\lambda_I\|_2)} \geq \frac{\delta(\log(p))^{\frac{1}{4}}\|\lambda_I\|_2^{\frac{1}{2}-\frac{\delta}{2}}\|\lambda_{I^*}\|_2^{\frac{\delta}{2}}}{\sqrt{K_0}}.$$

Obviously  $\sqrt{4\log(|I^*|) + 2\log(\log(p))} = o((\log(p))^{\frac{1}{4}}|I^*|^{\frac{\delta}{4}})$ , it follows that

$$\mathbb{P}(A_4(I)) \leq \mathbb{P}\left(\frac{\frac{\sqrt{2}\sum_{i \in I \cap I^*} \mu_i \tilde{U}_i (1 - \frac{\|\lambda_I\|_2}{\|\lambda_{I^*}\|_2})}{\sqrt{\frac{4\mu_{I \cap I^*}^T \Sigma_{I \cap I^*} \mu_{I \cap I^*} (\|\lambda_{I^*}\|_2 - \|\lambda_I\|_2^2)^2}{\|\lambda_I\|_2^2 \|\lambda_{I^*}\|_2^2}}} > \sqrt{4\log(|I^*|) + 2\log(\log(p))}\right).$$

Hence, by Lemma 2,

$$\mathbb{P}(A_4(I)) \leq \frac{1}{\sqrt{4\log(|I^*|) + 2\log(\log(p))}|I^*|^2 \log(p)} \leq \frac{1}{|I^*|^2 \log(p)}.$$

Therefore, note that  $\|\boldsymbol{\lambda}_{I^*}\|_2 \geq \|\boldsymbol{\lambda}_I\|_2$  implies that  $|I| \leq \|\boldsymbol{\lambda}_I\|_2^2/c^2 \leq \|\boldsymbol{\lambda}_{I^*}\|_2^2/c^2 \leq K_0^2|I^*|/c^2$ , we have

$$\begin{aligned}
\sum_{I \cap I^* \neq \emptyset} \mathbb{P}(A_4(I)) &= \sum_{\substack{I \cap I^* \neq \emptyset \\ \|\boldsymbol{\lambda}_I\|_2 \geq \|\boldsymbol{\lambda}_{I^*}\|_2}} \mathbb{P}(A_4(I)) + \sum_{\substack{I \cap I^* \neq \emptyset \\ \|\boldsymbol{\lambda}_I\|_2 < \|\boldsymbol{\lambda}_{I^*}\|_2}} \mathbb{P}(A_4(I)) \\
&\leq \frac{2L_{\max}^2}{L_{\max}^3 \log(p)} + \frac{1}{|I^*|^2 \log(p)} \sum_{i=1}^{K_0^2|I^*|/c^2} \{|I^*| + 2(i-1)\} \\
&= \frac{2 + K_0^2/c^2 + K_0^4/c^4}{\log(p)} = o(1)
\end{aligned} \tag{14}$$

Finally, we consider  $A_5(I)$ , by condition (E),

$$\text{Var} \left( \frac{\sum_{i \in I^* \setminus I} \mu_i \tilde{U}_i}{\|\boldsymbol{\lambda}_{I^*}\|_2} \right) = \frac{\boldsymbol{\mu}_{I^* \setminus I}^T \boldsymbol{\Sigma}_{I^* \setminus I} \boldsymbol{\mu}_{I^* \setminus I}}{\|\boldsymbol{\lambda}_{I^*}\|_2^2} \leq \frac{K_0 \|\boldsymbol{\mu}_{I^* \setminus I}\|_2^2}{\|\boldsymbol{\lambda}_{I^*}\|_2^2} \leq \frac{K_0 \|\boldsymbol{\mu}_{I^*}\|_2^2 \|\boldsymbol{\lambda}_{I^* \setminus I}\|_2^{1+\delta}}{\|\boldsymbol{\lambda}_{I^*}\|_2^{2+(1+\delta)}}.$$

It follows that

$$\frac{\frac{\|\boldsymbol{\mu}_{I^*}\|_2^2}{\|\boldsymbol{\lambda}_{I^*}\|_2^2} \left(1 - \frac{\|\boldsymbol{\lambda}_{I \cap I^*}\|_2^{1+\delta}}{\|\boldsymbol{\lambda}_{I^*}\|_2^\delta \|\boldsymbol{\lambda}_I\|_2}\right)}{\sqrt{\text{Var} \left( \frac{\sum_{i \in I^* \setminus I} \mu_i \tilde{U}_i}{\|\boldsymbol{\lambda}_{I^*}\|_2} \right)}} \geq \frac{\|\boldsymbol{\mu}_{I^*}\|_2 ( \|\boldsymbol{\lambda}_I\|_2 \|\boldsymbol{\lambda}_{I^*}\|_2^\delta - \|\boldsymbol{\lambda}_{I \cap I^*}\|_2^{1+\delta} ) \|\boldsymbol{\lambda}_{I^*}\|_2^{\frac{1-\delta}{2}}}{\sqrt{K_0} \|\boldsymbol{\lambda}_{I^* \setminus I}\|_2^{\frac{1+\delta}{2}} \|\boldsymbol{\lambda}_I\|_2}.$$

When  $|I^* \setminus I| > \frac{\eta_p}{2} |I^*|$ , by the former discussion,  $\frac{\|\boldsymbol{\lambda}_{I \cap I^*}\|_2^2}{\|\boldsymbol{\lambda}_{I^*}\|_2^2} \leq 1 - \frac{c^2 \eta_p}{2K_0^2}$  and thus

$$\begin{aligned}
\frac{\|\boldsymbol{\mu}_{I^*}\|_2 ( \|\boldsymbol{\lambda}_I\|_2 \|\boldsymbol{\lambda}_{I^*}\|_2^\delta - \|\boldsymbol{\lambda}_{I \cap I^*}\|_2^{1+\delta} ) \|\boldsymbol{\lambda}_{I^*}\|_2^{\frac{1-\delta}{2}}}{\sqrt{K_0} \|\boldsymbol{\lambda}_{I^* \setminus I}\|_2^{\frac{1+\delta}{2}} \|\boldsymbol{\lambda}_I\|_2} &\geq \frac{\|\boldsymbol{\mu}_{I^*}\|_2 \|\boldsymbol{\lambda}_{I^*}\|_2^{\frac{1-\delta}{2}} ( \|\boldsymbol{\lambda}_{I^*}\|_2^\delta - \|\boldsymbol{\lambda}_{I \cap I^*}\|_2^\delta )}{\sqrt{K_0} \|\boldsymbol{\lambda}_{I^* \setminus I}\|_2^{\frac{1+\delta}{2}}} \\
&\geq \frac{\|\boldsymbol{\mu}_{I^*}\|_2}{\sqrt{K_0}} \left\{ 1 - \left( \frac{\|\boldsymbol{\lambda}_{I \cap I^*}\|_2^2}{\|\boldsymbol{\lambda}_{I^*}\|_2^2} \right)^{\frac{\delta}{2}} \right\} \\
&\geq \frac{\|\boldsymbol{\mu}_{I^*}\|_2}{\sqrt{K_0}} \left\{ 1 - \left( \frac{c^2 \eta_p}{2K_0^2} \right)^{\frac{\delta}{2}} \right\} \\
&\geq \frac{\eta_p \delta c^2 \|\boldsymbol{\mu}_{I^*}\|_2}{4K_0^{\frac{5}{2}}} \geq \frac{\delta c^2 \eta_p |I^*|^{\frac{1}{4}} (\log(p))^{\frac{1}{4}}}{2\sqrt{2} K_0^{\frac{5}{2}}}.
\end{aligned}$$

Note that  $\sqrt{4 \log(L_{\max}) + 2 \log(\log(p))} = o(\eta_p \sqrt{\log(p)}) = o(\eta_p (\log(p))^{\frac{1}{4}} |I^*|^{\frac{1}{4}})$ , then by Lemma 2,

$$\mathbb{P}(A_5(I)) \leq \frac{1}{\sqrt{4 \log(L_{\max}) + 2 \log(\log(p))} L_{\max}^2 \log(p)} \leq \frac{1}{L_{\max}^2 \log(p)}$$

and hence

$$\sum_{I \cap I^* \neq \emptyset |I^* \setminus I| > \frac{\eta_p}{2} |I^*|} \mathbb{P}(A_5(I)) \leq \frac{2}{\log(p)}. \tag{15}$$

When  $|I \setminus I^*| > \frac{\eta_p}{2} |I^*|$ , by the former discussion, we have  $\frac{\|\lambda_I\|_2^2 - \|\lambda_{I \cap I^*}\|_2^2}{\|\lambda_I\|_2(\|\lambda_I\|_2 + \|\lambda_{I^*}\|_2)} \geq \frac{c^2 \eta_p}{6K_0^2}$  and thus

$$\begin{aligned}
\frac{\|\mu_{I^*}\|_2(\|\lambda_I\|_2\|\lambda_{I^*}\|_2^\delta - \|\lambda_{I \cap I^*}\|_2^{1+\delta})\|\lambda_{I^*}\|_2^{\frac{1-\delta}{2}}}{\sqrt{K_0}\|\lambda_{I^* \setminus I}\|_2^{\frac{1+\delta}{2}}\|\lambda_I\|_2} &\geq \frac{\|\mu_{I^*}\|_2}{\sqrt{K_0}} \times \frac{(\|\lambda_I\|_2 - \|\lambda_{I \cap I^*}\|_2)\|\lambda_{I^*}\|_2^{\frac{1+\delta}{2}}}{\|\lambda_{I^* \setminus I}\|_2^{\frac{1+\delta}{2}}\|\lambda_I\|_2} \\
&\geq \frac{\|\mu_{I^*}\|_2}{\sqrt{K_0}} \times \frac{\|\lambda_I\|_2^2 - \|\lambda_{I \cap I^*}\|_2^2}{\|\lambda_I\|_2(\|\lambda_{I^*}\|_2 + \|\lambda_I\|_2)} \\
&\geq \frac{c^2 \eta_p \|\mu_{I^*}\|_2}{6K_0^{\frac{5}{2}}} \geq \frac{c^2 \eta_p}{6K_0^{\frac{5}{2}}} \|\lambda_{I^*}\|_2 \sqrt{\log(p)}.
\end{aligned}$$

Note that  $\sqrt{4 \log(L_{\max}) + 2 \log(\log(p))} = o(\eta_p \sqrt{\log(p)}) = o(\eta_p (\log(p))^{\frac{1}{4}} |I^*|^{\frac{1}{4}})$ , then by Lemma 2,

$$\mathbb{P}(A_5(I)) \leq \frac{1}{\sqrt{4 \log(L_{\max}) + 2 \log(\log(p))} L_{\max}^2 \log(p)} \leq \frac{1}{L_{\max}^2 \log(p)}$$

and hence

$$\sum_{I \cap I^* \neq \emptyset, |I \setminus I^*| > \frac{\eta_p}{2} |I^*|} \mathbb{P}(A_5(I)) \leq \frac{2}{\log(p)}. \quad (16)$$

Therefore, by (7) and (9)-(16), we have

$$\mathbb{P}(J(\hat{I}, I^*) < 1 - \eta_p, \hat{I} \cap I^* \neq \emptyset) = o(1).$$

Combine with (5) and (6), we complete the proof.  $\square$

## 2 Supplementary Figures

Figure S1: Power and accuracy of estimated signal region comparisons of Q-SCAN and M-SCAN. We evaluated power via the signal region detection rate and the Jaccard index defined in the simulation section. Both criteria were calculated at the family-wise error rate at 0.05 level. The number of variants in signal region  $p_0$  was randomly select between 50 and 80. The sparsity index  $\xi = 3/4$  and  $s = p_0^\xi$  causal variants were selected randomly within each signal region. Each of causal variant has an effect size as a decreasing function of MAF,  $\beta = c \log_{10}(\text{MAF})$  and  $c = 0.14$ . From left to right, the plots consider settings in which the coefficients for the causal rare variants are 100% positive (0% negative), 80% positive (20% negative), and 50% positive (50% negative). We repeated the simulation for 1000 times. Q-SCAN and M-SCAN refer to the scan procedures using the scan statistics  $\sum_{i \in I} U_i^2 - \mathbb{E}(\sum_{i \in I} U_i^2)/\text{var}(\sum_{i \in I} U_i^2)$  and  $(\sum_{i \in I} U_i)^2/\text{var}(\sum_{i \in I} U_i)$ , respectively. In both two scan procedure, the range of variants number in searching windows was between 40 and 200.

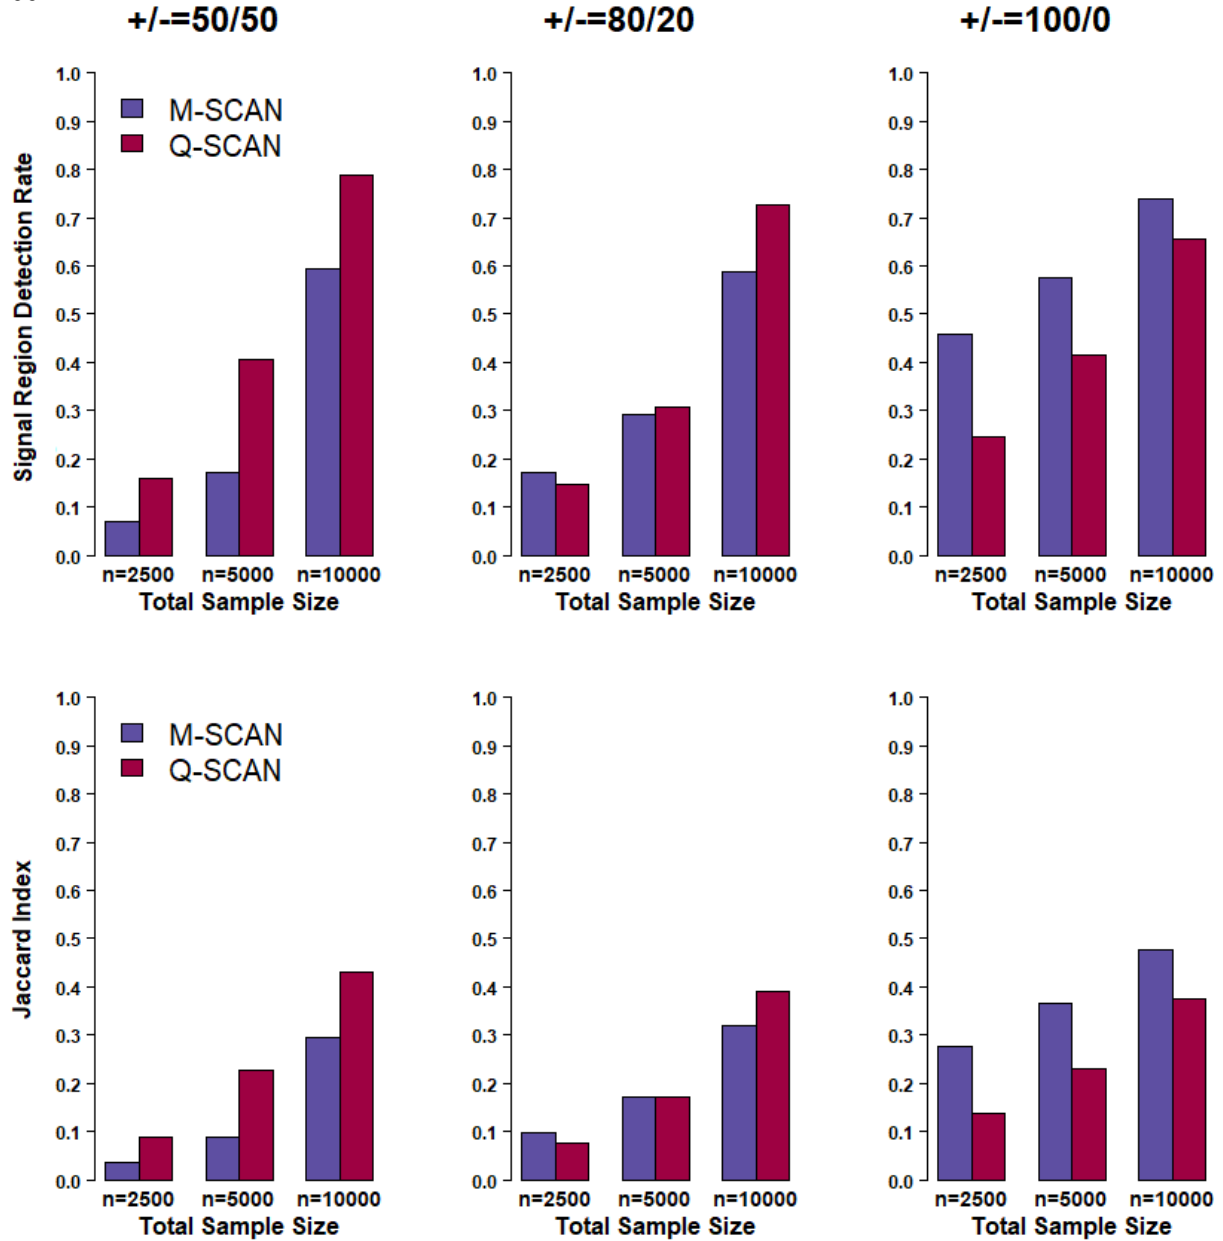



Figure S2: Power and accuracy of estimated signal region comparisons of Q-SCAN and M-SCAN for multiple effects. We evaluated power via the signal region detection rate and the Jaccard index defined in the simulation section. Both criteria were calculated at the family-wise error rate at 0.05 level. The number of variants in signal region  $p_0$  was randomly select between 50 and 80. The sparsity index  $\xi = 2/3$  and  $s = p_0^\xi$  causal variants were selected randomly within each signal region. Each of causal variant has an effect size as a decreasing function of MAF,  $\beta = c \log_{10}(\text{MAF})$ . The value  $c$  varies from 0.11 to 0.31. From left to right, the plots consider settings in which the coefficients for the causal rare variants are 100% positive (0% negative), 80% positive (20% negative), and 50% positive (50% negative). We repeated the simulation for 1000 times. Q-SCAN and M-SCAN refer to the scan procedures using the scan statistics  $\sum_{i \in I} U_i^2 - \mathbb{E}(\sum_{i \in I} U_i^2)/\text{var}(\sum_{i \in I} U_i^2)$  and  $(\sum_{i \in I} U_i)^2/\text{var}(\sum_{i \in I} U_i)$ , respectively. In both two scan procedure, the range of variants number in searching windows was between 40 and 200.

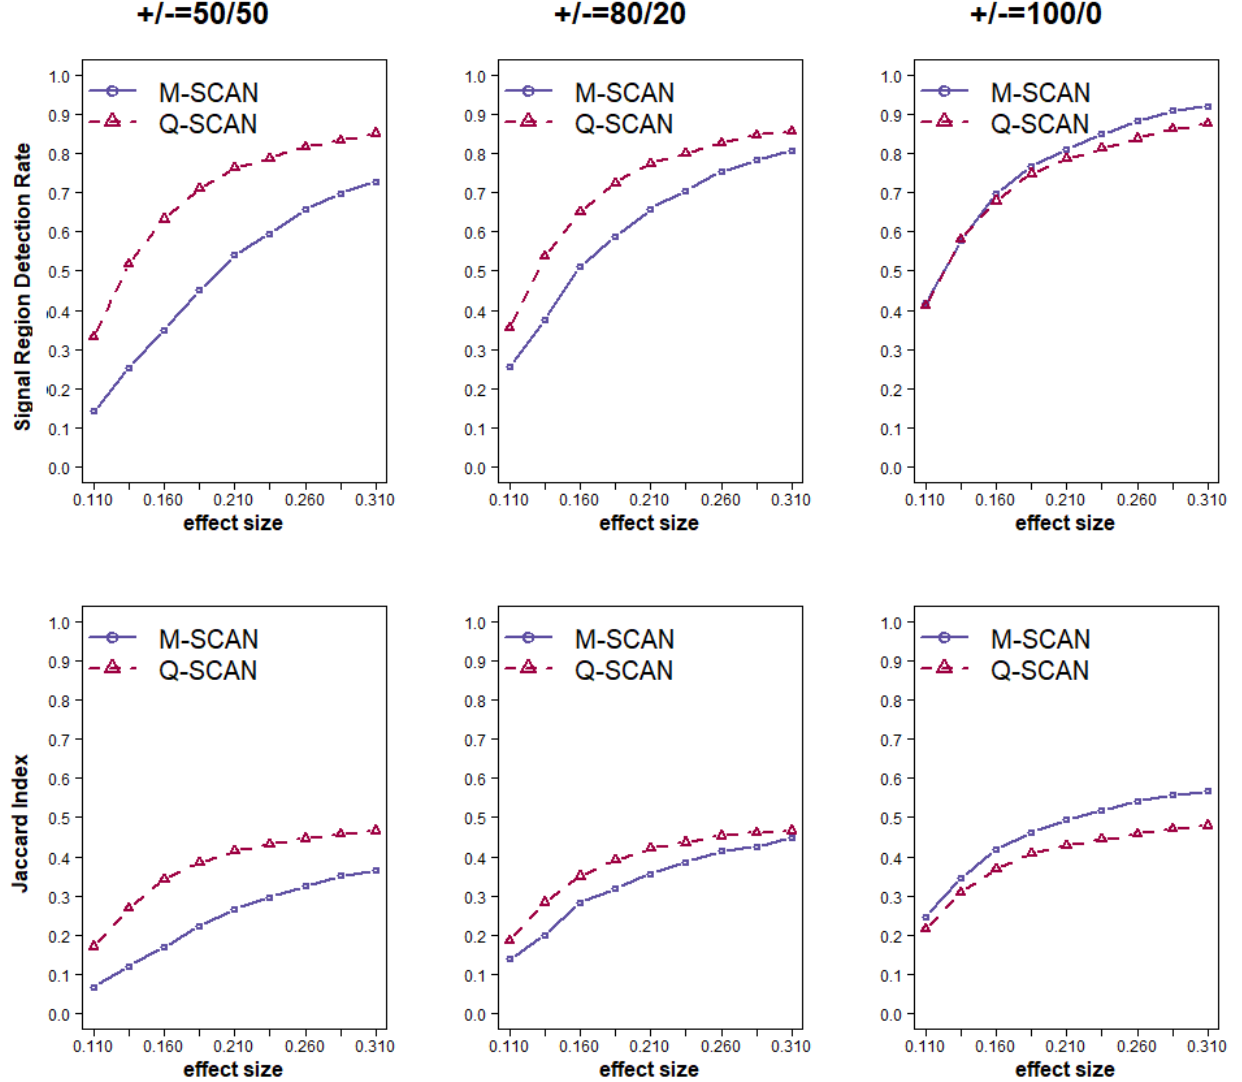

Figure S3: Power and accuracy of estimated signal region comparisons of Q-SCAN and M-SCAN for multiple effects.. We evaluated power via the signal region detection rate and the Jaccard index defined in the simulation section. Both criteria were calculated at the family-wise error rate at 0.05 level. The number of variants in signal region  $p_0$  was randomly select between 50 and 80. The sparsity index  $\xi = 1/2$  and  $s = p_0^\xi$  causal variants were selected randomly within each signal region. Each of causal variant has an effect size as a decreasing function of MAF,  $\beta = c \log_{10}(\text{MAF})$ . The value  $c$  varies from 0.15 to 0.39. From left to right, the plots consider settings in which the coefficients for the causal rare variants are 100% positive (0% negative), 80% positive (20% negative), and 50% positive (50% negative). We repeated the simulation for 1000 times. Q-SCAN and M-SCAN refer to the scan procedures using the scan statistics  $\sum_{i \in I} U_i^2 - \mathbb{E}(\sum_{i \in I} U_i^2)/\text{var}(\sum_{i \in I} U_i^2)$  and  $(\sum_{i \in I} U_i)^2/\text{var}(\sum_{i \in I} U_i)$ , respectively. In both two scan procedure, the range of variants number in searching windows was between 40 and 200.

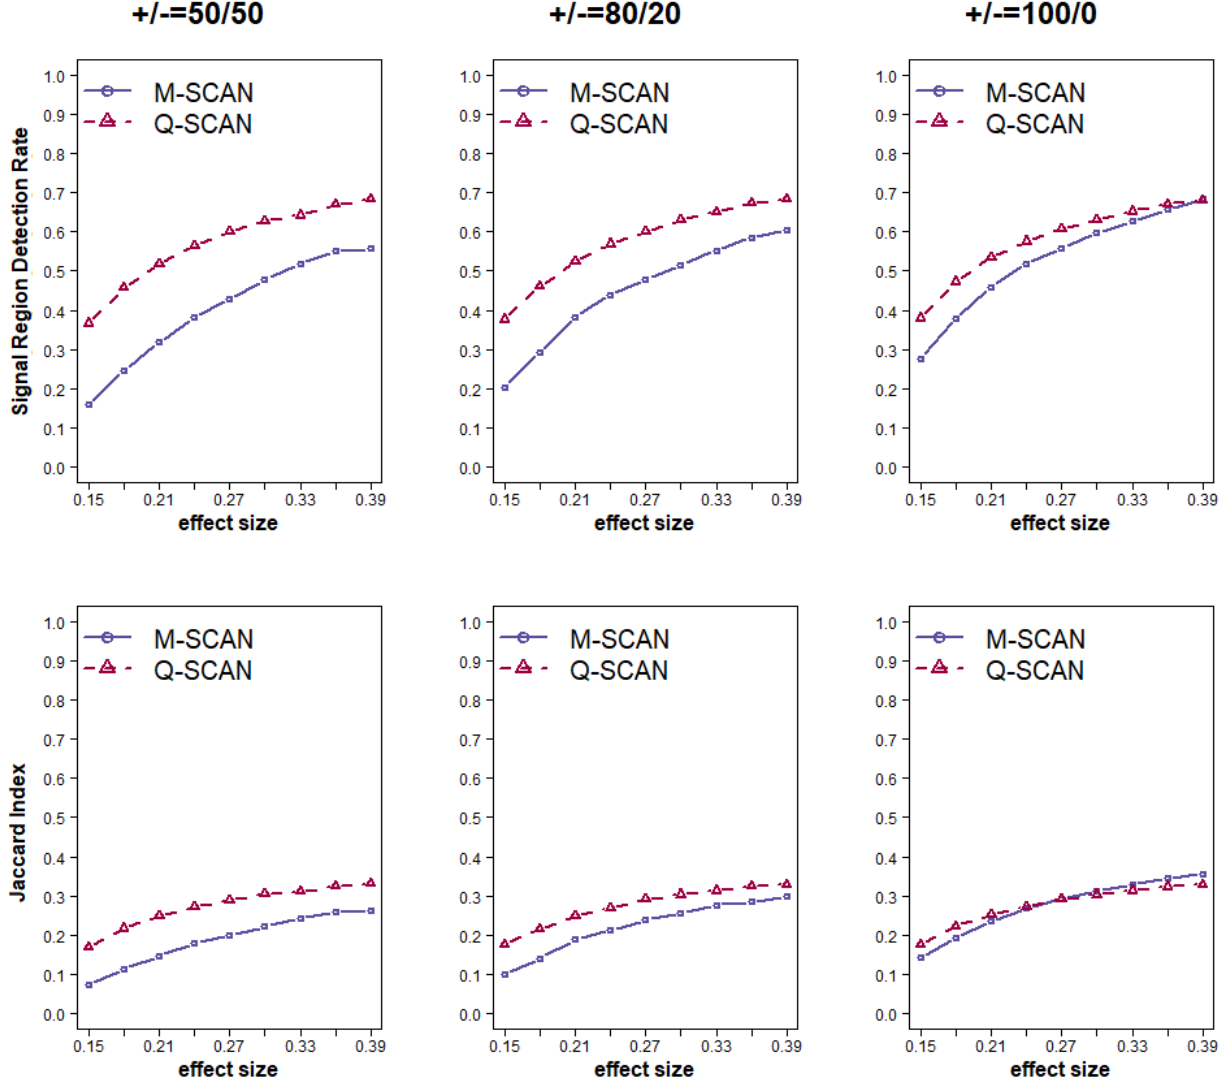

Figure S4: Power and accuracy of estimated signal region comparisons of Q-SCAN and M-SCAN for multiple effects.. We evaluated power via the signal region detection rate and the Jaccard index defined in the simulation section. Both criteria were calculated at the family-wise error rate at 0.05 level. The number of variants in signal region  $p_0$  was randomly select between 50 and 80. The sparsity index  $\xi = 3/4$  and  $s = p_0^\xi$  causal variants were selected randomly within each signal region. Each of causal variant has an effect size as a decreasing function of MAF,  $\beta = c \log_{10}(\text{MAF})$ . The value  $c$  varies from 0.09 to 0.17. From left to right, the plots consider settings in which the coefficients for the causal rare variants are 100% positive (0% negative), 80% positive (20% negative), and 50% positive (50% negative). We repeated the simulation for 1000 times. Q-SCAN and M-SCAN refer to the scan procedures using the scan statistics  $\sum_{i \in I} U_i^2 - \mathbb{E}(\sum_{i \in I} U_i^2)/\text{var}(\sum_{i \in I} U_i^2)$  and  $(\sum_{i \in I} U_i)^2/\text{var}(\sum_{i \in I} U_i)$ , respectively. In both two scan procedure, the range of variants number in searching windows was between 40 and 200.

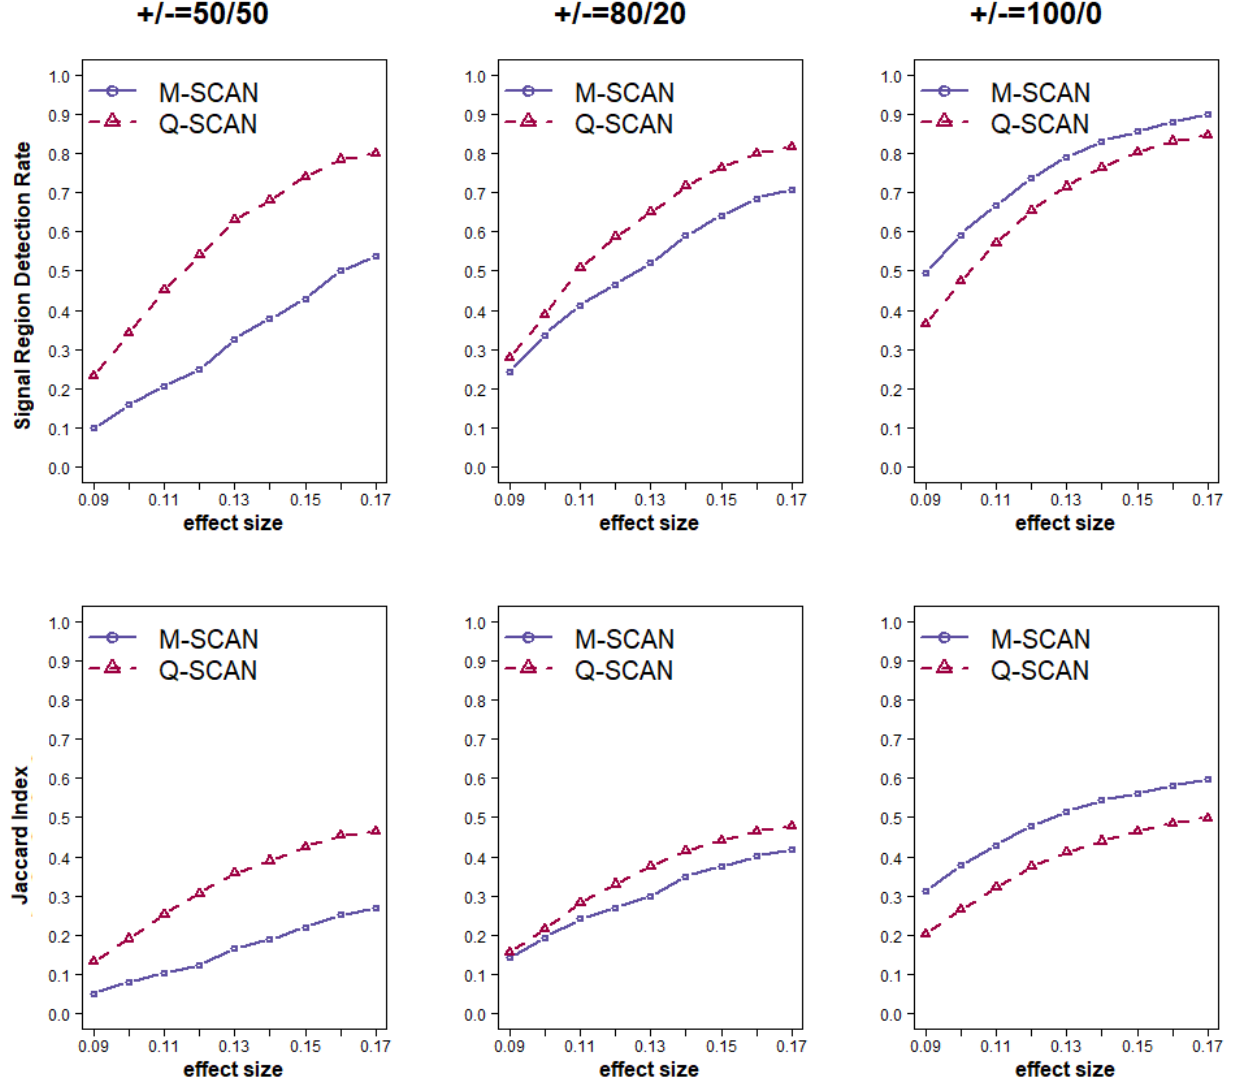

Figure S5: Distribution of small, dense, low-density lipoprotein cholesterol (LDL) and inverse rank-normal transformed LDL among AAs and EAs in ARIC data.

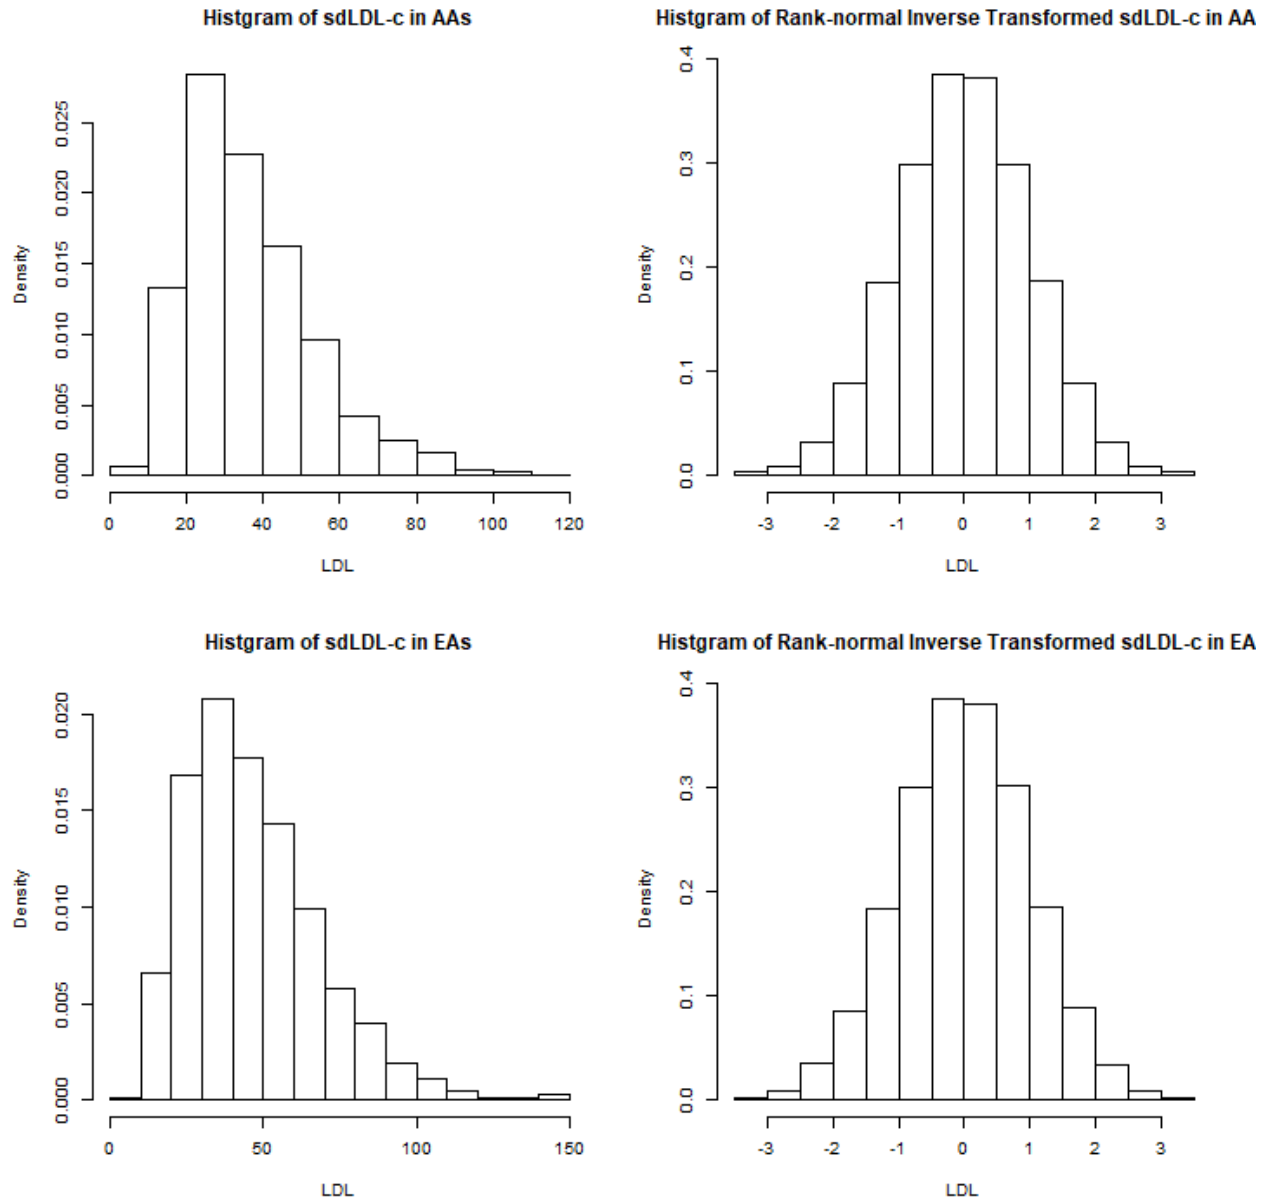

Figure S6: Distribution of neutrophil count and inverse rank-normal transformed neutrophil count among AAs and EAs in ARIC data.

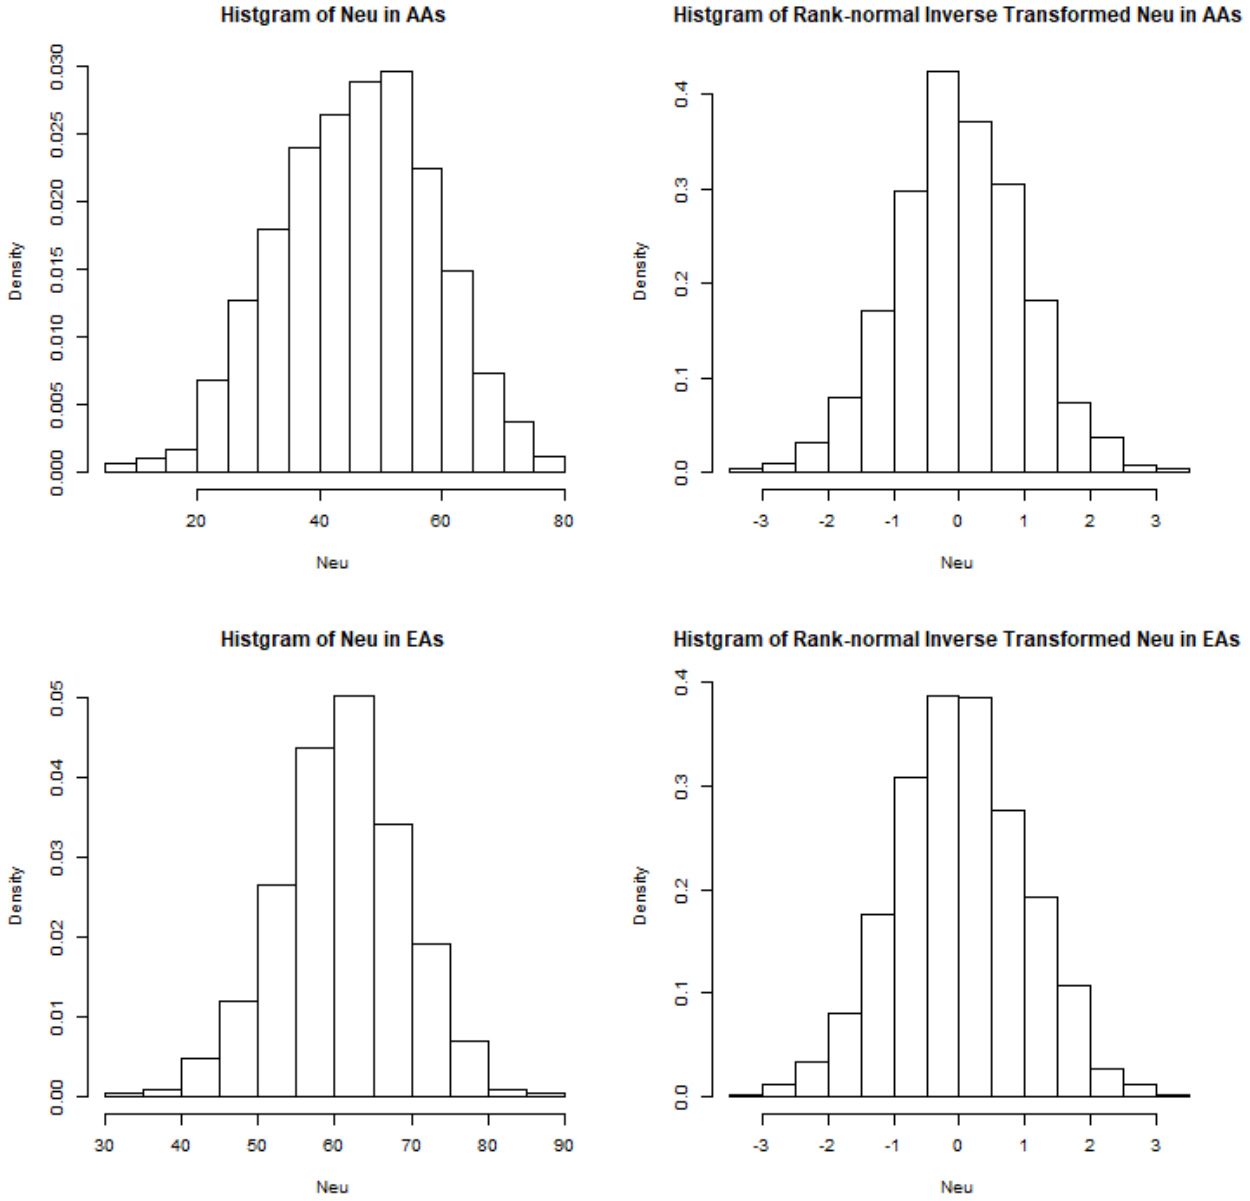

### 3 Supplementary Tables

Table S1: Regions that are significantly associated with neutrophil counts among African Americans in ARIC WGS study detected by Q-SCAN. FWER represent the empirical genome-wide family-wise error rate. A region is significant if its FWER smaller than 0.05. The physical positions of the windows are based on build hg19.

| Chr | Start Pos.  | End Pos.    | Length (bp) | # SNPs | FWER   |
|-----|-------------|-------------|-------------|--------|--------|
| 1   | 155,064,139 | 155,068,456 | 4,318       | 42     | 0.0065 |
| 1   | 156,116,488 | 156,119,540 | 3,053       | 40     | 0.0275 |
| 1   | 156,747,349 | 156,749,487 | 2,139       | 42     | 0.0005 |
| 1   | 156,757,680 | 156,760,860 | 3,181       | 40     | 0.004  |
| 1   | 156,785,778 | 156,788,247 | 2,470       | 40     | 0.0005 |
| 1   | 157,076,362 | 157,078,699 | 2,338       | 45     | 0.0075 |
| 1   | 157,395,570 | 157,398,264 | 2,695       | 40     | 0.0335 |
| 1   | 157,402,513 | 157,404,607 | 2,095       | 40     | 0.003  |
| 1   | 157,414,963 | 157,416,332 | 1,370       | 40     | 0.006  |
| 1   | 157,452,612 | 157,455,395 | 2,784       | 40     | 0.028  |
| 1   | 157,672,259 | 157,675,671 | 3,413       | 40     | 0.007  |
| 1   | 157,955,804 | 157,959,966 | 4,163       | 67     | 0.01   |
| 1   | 158,730,560 | 158,733,423 | 2,864       | 40     | 0.0005 |
| 1   | 159,159,041 | 159,173,539 | 14,499      | 192    | 0.0005 |
| 1   | 159,174,123 | 159,177,323 | 3,201       | 48     | 0      |
| 1   | 159,203,085 | 159,206,332 | 3,248       | 40     | 0.0005 |
| 1   | 159,222,723 | 159,225,507 | 2,785       | 40     | 0.0005 |
| 1   | 159,290,525 | 159,294,814 | 4,290       | 41     | 0      |
| 1   | 159,311,607 | 159,317,891 | 6,285       | 79     | 0.0015 |
| 1   | 159,326,579 | 159,330,161 | 3,583       | 40     | 0      |
| 1   | 159,336,948 | 159,340,299 | 3,352       | 52     | 0.0055 |
| 1   | 159,368,937 | 159,372,815 | 3,879       | 53     | 0      |
| 1   | 159,377,099 | 159,385,359 | 8,261       | 162    | 0.0285 |
| 1   | 159,392,547 | 159,397,122 | 4,576       | 60     | 0.0005 |
| 1   | 159,402,756 | 159,405,840 | 3,085       | 40     | 0.001  |
| 1   | 159,410,752 | 159,413,898 | 3,147       | 40     | 0      |
| 1   | 159,428,631 | 159,431,795 | 3,165       | 40     | 0.0005 |
| 1   | 159,445,655 | 159,449,083 | 3,429       | 46     | 0      |
| 1   | 159,449,926 | 159,453,749 | 3,824       | 55     | 0.0005 |
| 1   | 159,477,947 | 159,491,638 | 13,692      | 154    | 0      |
| 1   | 159,501,094 | 159,508,010 | 6,917       | 88     | 0      |
| 1   | 159,513,613 | 159,517,170 | 3,558       | 41     | 0      |
| 1   | 159,535,940 | 159,543,770 | 7,831       | 140    | 0      |
| 1   | 159,546,141 | 159,550,007 | 3,867       | 45     | 0      |
| 1   | 159,556,355 | 159,561,758 | 5,404       | 74     | 0.014  |
| 1   | 159,571,615 | 159,573,805 | 2,191       | 40     | 0.0195 |
| 1   | 159,709,610 | 159,711,987 | 2,378       | 40     | 0.006  |
| 1   | 159,801,023 | 159,803,453 | 2,431       | 40     | 0      |
| 1   | 160,113,613 | 160,117,505 | 3,893       | 40     | 0      |
| 1   | 160,638,498 | 160,640,762 | 2,265       | 41     | 0.0255 |
| 1   | 161,650,448 | 161,652,574 | 2,127       | 40     | 0.0275 |
| 1   | 161,663,548 | 161,667,036 | 3,489       | 40     | 0.001  |

Table S2: Regions that are significantly associated with neutrophil counts among African Americans in ARIC WGS study detected by M-SCAN. FWER represent the empirical genome-wide family-wise error rate. A region is significant if its FWER smaller than 0.05. The physical positions of the windows are based on build hg19.

| Chr | Start Pos.  | End Pos.    | Length (bp) | # SNPs | FWER   |
|-----|-------------|-------------|-------------|--------|--------|
| 1   | 159,167,097 | 159,173,539 | 6,443       | 93     | 0      |
| 1   | 159,174,002 | 159,177,323 | 3,322       | 51     | 0      |
| 1   | 159,222,723 | 159,225,507 | 2,785       | 40     | 0      |
| 1   | 159,291,683 | 159,295,534 | 3,852       | 45     | 0      |
| 1   | 159,317,009 | 159,319,877 | 2,869       | 56     | 0      |
| 1   | 159,325,743 | 159,329,281 | 3,539       | 41     | 0.0265 |
| 1   | 159,372,133 | 159,374,293 | 2,161       | 40     | 0.005  |
| 1   | 159,404,803 | 159,408,308 | 3,506       | 50     | 0      |
| 1   | 159,410,975 | 159,414,384 | 3,410       | 47     | 0      |
| 1   | 159,419,602 | 159,424,587 | 4,986       | 119    | 0.009  |
| 1   | 159,446,104 | 159,449,083 | 2,980       | 43     | 0      |
| 1   | 159,453,205 | 159,456,681 | 3,477       | 49     | 0      |
| 1   | 159,477,411 | 159,484,884 | 7,474       | 60     | 0      |
| 1   | 159,501,163 | 159,509,358 | 8,196       | 116    | 0.0005 |
| 1   | 159,513,592 | 159,517,653 | 4,062       | 44     | 0      |
| 1   | 159,536,458 | 159,543,683 | 7,226       | 127    | 0.007  |
| 1   | 159,546,317 | 159,551,128 | 4,812       | 54     | 0      |
| 1   | 159,556,077 | 159,558,783 | 2,707       | 40     | 0.03   |
| 1   | 161,663,297 | 161,666,633 | 3337        | 42     | 0      |

Table S3: Regions that are significantly associated with neutrophil counts among African Americans in ARIC WGS study detected by sliding window procedure using SKAT. A region is significant if its p-value is small than  $3.75 \times 10^{-8}$ , which control the FWER at 0.05 level by Bonferroni correction. The physical positions of the windows are based on build hg19.

| Chr | Start Pos.  | End Pos.    | Length (bp) | # SNPs | p-value                |
|-----|-------------|-------------|-------------|--------|------------------------|
| 1   | 155,052,150 | 155,056,149 | 4,000       | 38     | $3.67 \times 10^{-8}$  |
| 1   | 156,746,150 | 156,750,149 | 4,000       | 60     | $4.57 \times 10^{-9}$  |
| 1   | 158,572,150 | 158,576,149 | 4,000       | 46     | $1.67 \times 10^{-8}$  |
| 1   | 158,730,150 | 158,734,149 | 4,000       | 48     | $3.26 \times 10^{-8}$  |
| 1   | 158764150   | 158768149   | 4,000       | 39     | $8.71 \times 10^{-12}$ |
| 1   | 159,166,150 | 159,170,149 | 4,000       | 57     | $1.10 \times 10^{-9}$  |
| 1   | 159,168,150 | 159,172,149 | 4,000       | 62     | $2.80 \times 10^{-11}$ |
| 1   | 159,170,150 | 159,174,149 | 4,000       | 64     | $1.86 \times 10^{-9}$  |
| 1   | 159,172,150 | 159,176,149 | 4,000       | 57     | $2.79 \times 10^{-10}$ |
| 1   | 159,174,150 | 159,178,149 | 4,000       | 56     | $4.11 \times 10^{-11}$ |
| 1   | 159,176,150 | 159,180,149 | 4,000       | 53     | $7.62 \times 10^{-9}$  |
| 1   | 159,288,150 | 159,292,149 | 4,000       | 42     | $2.21 \times 10^{-10}$ |
| 1   | 159,290,150 | 159,294,149 | 4,000       | 38     | $3.61 \times 10^{-14}$ |
| 1   | 159,324,150 | 159,328,149 | 4,000       | 45     | $1.55 \times 10^{-8}$  |
| 1   | 159,336,150 | 159,340,149 | 4,000       | 56     | $2.86 \times 10^{-8}$  |
| 1   | 159,370,150 | 159,374,149 | 4,000       | 60     | $2.42 \times 10^{-11}$ |
| 1   | 159,402,150 | 159,406,149 | 4,000       | 57     | $7.70 \times 10^{-11}$ |
| 1   | 159,408,150 | 159,412,149 | 4,000       | 59     | $9.42 \times 10^{-11}$ |
| 1   | 159,410,150 | 159,414,149 | 4,000       | 53     | $7.45 \times 10^{-9}$  |
| 1   | 159,416,150 | 159,420,149 | 4,000       | 102    | $1.18 \times 10^{-9}$  |
| 1   | 159,418,150 | 159,422,149 | 4,000       | 98     | $9.47 \times 10^{-9}$  |
| 1   | 159,436,150 | 159,440,149 | 4,000       | 42     | $3.12 \times 10^{-8}$  |
| 1   | 159,442,150 | 159,446,149 | 4,000       | 61     | $4.99 \times 10^{-10}$ |
| 1   | 159,444,150 | 159,448,149 | 4,000       | 65     | $4.56 \times 10^{-11}$ |
| 1   | 159,446,150 | 159,450,149 | 4,000       | 62     | $1.87 \times 10^{-16}$ |
| 1   | 159,448,150 | 159,452,149 | 4,000       | 53     | $2.15 \times 10^{-10}$ |
| 1   | 159,450,150 | 159,454,149 | 4,000       | 50     | $5.13 \times 10^{-15}$ |
| 1   | 159,452,150 | 159,456,149 | 4,000       | 53     | $6.52 \times 10^{-10}$ |
| 1   | 159,456,150 | 159,460,149 | 4,000       | 49     | $2.77 \times 10^{-8}$  |
| 1   | 159,468,150 | 159,472,149 | 4,000       | 44     | $7.48 \times 10^{-9}$  |
| 1   | 159,470,150 | 159,474,149 | 4,000       | 46     | $6.28 \times 10^{-11}$ |
| 1   | 159,476,150 | 159,480,149 | 4,000       | 29     | $8.48 \times 10^{-9}$  |
| 1   | 159,478,150 | 159,482,149 | 4,000       | 26     | $7.02 \times 10^{-11}$ |
| 1   | 159,482,150 | 159,486,149 | 4,000       | 44     | $3.52 \times 10^{-10}$ |
| 1   | 159,484,150 | 159,488,149 | 4,000       | 58     | $2.36 \times 10^{-13}$ |
| 1   | 159,486,150 | 159,490,149 | 4,000       | 58     | $1.25 \times 10^{-12}$ |
| 1   | 159,488,150 | 159,492,149 | 4,000       | 54     | $9.74 \times 10^{-14}$ |
| 1   | 159,490,150 | 159,494,149 | 4,000       | 48     | $1.01 \times 10^{-11}$ |
| 1   | 159,492,150 | 159,496,149 | 4,000       | 31     | $3.33 \times 10^{-9}$  |



| Chr | Start Pos.  | End Pos.    | Length (bp) | # SNPs | p-value                |
|-----|-------------|-------------|-------------|--------|------------------------|
| 1   | 159,500,150 | 159,504,149 | 4,000       | 44     | $1.16 \times 10^{-12}$ |
| 1   | 159,502,150 | 159,506,149 | 4,000       | 54     | $7.96 \times 10^{-16}$ |
| 1   | 159,504,150 | 159,508,149 | 4,000       | 57     | $5.01 \times 10^{-14}$ |
| 1   | 159,506,150 | 159,510,149 | 4,000       | 70     | $4.56 \times 10^{-10}$ |
| 1   | 159,512,150 | 159,516,149 | 4,000       | 70     | $1.94 \times 10^{-9}$  |
| 1   | 159,514,150 | 159,518,149 | 4,000       | 44     | $8.65 \times 10^{-13}$ |
| 1   | 159,518,150 | 159,522,149 | 4,000       | 58     | $1.14 \times 10^{-8}$  |
| 1   | 159,520,150 | 159,524,149 | 4,000       | 39     | $2.26 \times 10^{-11}$ |
| 1   | 159,534,150 | 159,538,149 | 4,000       | 43     | $3.41 \times 10^{-10}$ |
| 1   | 159,536,150 | 159,540,149 | 4,000       | 65     | $3.85 \times 10^{-11}$ |
| 1   | 159,538,150 | 159,542,149 | 4,000       | 71     | $1.16 \times 10^{-9}$  |
| 1   | 159,540,150 | 159,544,149 | 4,000       | 82     | $4.68 \times 10^{-10}$ |
| 1   | 159,542,150 | 159,546,149 | 4,000       | 107    | $3.42 \times 10^{-8}$  |
| 1   | 159,546,150 | 159,550,149 | 4,000       | 45     | $8.35 \times 10^{-14}$ |
| 1   | 159,548,150 | 159,552,149 | 4,000       | 45     | $8.14 \times 10^{-16}$ |
| 1   | 159,556,150 | 159,560,149 | 4,000       | 57     | $1.19 \times 10^{-13}$ |
| 1   | 159,558,150 | 159,562,149 | 4,000       | 60     | $4.82 \times 10^{-9}$  |
| 1   | 159,576,150 | 159,580,149 | 4,000       | 50     | $2.87 \times 10^{-8}$  |
| 1   | 159,580,150 | 159,584,149 | 4,000       | 73     | $5.16 \times 10^{-10}$ |
| 1   | 159,798,150 | 159,802,149 | 4,000       | 83     | $6.31 \times 10^{-13}$ |
| 1   | 159,800,150 | 159,804,149 | 4,000       | 61     | $3.93 \times 10^{-10}$ |
| 1   | 161,506,150 | 161,510,149 | 4,000       | 90     | $3.06 \times 10^{-8}$  |
| 1   | 161,508,150 | 161,512,149 | 4,000       | 91     | $9.30 \times 10^{-10}$ |

## References

- Laurent, B. and Massart, P. (2000). Adaptive estimation of a quadratic functional by model selection. *Annals of Statistics*, pages 1302–1338.
- Petrov, V. (1968). Asymptotic behavior of probabilities of large deviations. *Theory of Probability & Its Applications*, 13(3):408–420.
